# Supplementary material for: Universal motion of mirror-symmetric microparticles in confined Stokes flow
Source: arXiv:2003.02806 ancillary file (2020-03-16)
Supplement: Supplementary file 1 [file Supplementary_Information.pdf]

# Supplementary Information for

## Universal motion of mirror-symmetric microparticles in confined Stokes flow

**R. N. Georgiev, S. O. Toscano, W. E. Uspal, B. Bet, S. Samin, R. van Roij and H. B. Eral**

**Huseyin Burak Eral**
**E-mail: H.B.Eral@tudelft.nl**

### This PDF file includes:

Supplementary text
Figs. S1 to S19
Table S1
SI References

## Supporting Information Text

## 1. Particle trajectory in confined Stokes flow

We recently obtained expressions for the rotation and drift of a mirror-symmetric particle in confined Stokes flow (1). Here, we summarize this derivation by highlighting the main assumptions and underlying concepts. Even though our focus is particles with a single mirror plane, we complement the discussion by considering objects with zero, two and four mirror planes and demonstrate how symmetry determines their dynamics. For brevity, we refer to the longitudinal and transversal force along with the in-plane torque as 'forces' throughout this supplementary note. Likewise, we will not explicitly distinguish between the linear and angular velocities.

We start deriving the equations of motion (equations 2 and 3 in the main text), by first considering a particle subjected to two-dimensional creeping flow in an infinitely large domain with no confining plates. To account for the strong confinement both the particle and the flow experience, we implicitly add the drag from the top and bottom channel walls. Our treatment does not include the side walls of the channel and, consequently, we neglect repulsion between the particle and its hydrodynamic image in their vicinity.

As creeping flow is instantaneous, we assume the particle is force-free at any instance in time and the flow adjusts immediately to any change in its orientation or position. We couple this assumption to the Stokes linearity principle, which decomposes the force on a moving particle subjected to flow into a force on a stationary particle in flow and a force on a moving particle in quiescent fluid. Mathematically, we express this force balance through particle and flow velocities via the *resistance tensor*, a linear operator that transforms velocity into force. Introduced by Howard Brenner (2), the resistance tensor generalizes the concept of the drag coefficient and gives a mathematical explanation for the lift and torque experienced by a anisotropic particles sedimenting under gravity. The following pedagogical review serves as an introduction to microhydrodynamics and provides context for our later discussions.

**A. Resistance tensor.** Similarly to the way the stress tensor expresses how a fluid resists deformation, the resistance tensor $\mathsf{R}_\mathrm{p}$ represents how a stationary fluid resists the motion of a particle and relates the velocity of the particle to the hydrodynamic forces acting on it. The columns of the resistance tensor for a particle with orientation $\theta$ are given by the forces acting on it as it exhibits only one degree of freedom. Explicitly, we first set the $x-$velocity of the particle to unity $\dot{x}=1$, while keeping $\left(\dot{y},\dot{\theta}\right)=(0,0)$ and obtain the forces acting on it. Next, we prescribe $\dot{y}=1$, while $\left(\dot{x},\dot{\theta}\right)=(0,0)$, yielding the second column of the resistance tensor. We complete the resistance tensor with the forces acting on a particle, which only rotates $\left(\dot{x},\dot{y},\dot{\theta}\right)=(0,0,1)$:

$$\mathsf{R}_\mathrm{p}\left(\theta\right)=-\begin{pmatrix} F_x\left(1,0,0\right) & F_x\left(0,1,0\right) & F_x\left(0,0,1\right)\\ F_y\left(1,0,0\right) & F_y\left(0,1,0\right) & F_y\left(0,0,1\right)\\ T_z\left(1,0,0\right) & T_z\left(0,1,0\right) & T_z\left(0,0,1\right)\end{pmatrix} \qquad [1]$$

Throughout this discussion we neglect the influence of side walls on the particle. Hence, the resistance tensor does not depend on the position of the particle and is only influenced by its orientation.

Due to the linearity of Stokes flow this velocity-to-force relation is linear:

$$\begin{pmatrix} F_x\\ F_y\\ T_z\end{pmatrix}=-\eta\mathsf{R}_\mathrm{p}\left(\theta\right)\cdot\begin{pmatrix}\dot{x}\\ \dot{y}\\ \dot{\theta}\end{pmatrix} \qquad [2]$$

As an example, we present the resistance tensor of a mirror-symmetric particle, whose long axis is neither parallel, nor normal to the flow in Fig. S1. As one such anisotropic particle moves through a quiescent fluid, the anisotropic disturbances it creates result in net forces and torque acting on it. The off-diagonal elements of $\mathsf{R}_\mathrm{p}$ quantify the coupling of the modes of motion – even if the particle were to move only to the right at a given instance in time, it would not only experience drag, but also an anticlockwise torque and a positive force along $y$ (Fig. S1).

Furthermore, knowing $\mathsf{R}_\mathrm{p}\left(\theta\right)$ enables the efficient calculation of the hydrodynamic forces for any orientation $\theta+\Delta\theta$ by rotating the resistance tensor. To do so, we can follow Brenner's approach of decomposing $\mathsf{R}_\mathrm{p}\left(\theta\right)$ into a translation tensor $\mathsf{R}_\mathrm{p,T}\left(\theta\right)$, a rotation tensor $\mathsf{R}_\mathrm{p,R}\left(\theta\right)$ and two coupling tensors $\mathsf{R}_\mathrm{p,C}\left(\theta\right)$ and $\mathsf{R}^\intercal_\mathrm{p,C}\left(\theta\right)$:

$$\mathsf{R}_\mathrm{p}\left(\theta\right)=\begin{pmatrix}\mathsf{R}_\mathrm{p,T}\left(\theta\right) & \mathsf{R}_\mathrm{p,C}\left(\theta\right)\\ \mathsf{R}^\intercal_\mathrm{p,C}\left(\theta\right) & \mathsf{R}_\mathrm{p,R}\left(\theta\right)\end{pmatrix} \qquad [3]$$

The translation and rotation tensors are square matrices with size equal to the number of translational and rotational degrees of freedom the particle exhibits, while the size of the coupling tensors is such as to make the resistance tensor a square matrix. For example, a 3D particle, exhibiting three translations and three rotations, has a 6-by-6 resistance tensor composed of four square matrices of size 3. As one of the translations and two of the rotations are cancelled in two dimensions, two-dimensional particles have resistance tensors of size 3, comprising a 2-by-2 translation matrix, a 1-by-1 rotation matrix and two coupling vectors of size 2. To obtain the resistance tensor at any orientation, we rotate the translation and coupling tensors of $\mathsf{R}_\mathrm{p}\left(\theta\right)$:

$$\mathsf{R}_\mathrm{p}\left(\theta+\Delta\theta\right)=\begin{pmatrix}\mathsf{M}\cdot\mathsf{R}_\mathrm{p,T}\left(\theta\right)\cdot\mathsf{M}^\intercal & \mathsf{M}\cdot\mathsf{R}_\mathrm{p,C}\left(\theta\right)\\ \mathsf{M}\cdot\mathsf{R}^\intercal_\mathrm{p,C}\left(\theta\right) & \mathsf{R}_\mathrm{p,R}\left(\theta\right)\end{pmatrix},\text{where } \mathsf{M}=\begin{pmatrix}\cos\Delta\theta & -\sin\Delta\theta\\ \sin\Delta\theta & \cos\Delta\theta\end{pmatrix} \qquad [4]$$

Thus, computing the resistance tensor of a particle with an arbitrary orientation in an unbound fluid, in fact, yields the resistance tensors for any orientation.

**B. Force- and torque-free velocities of a particle in confined Stokes flow.** Up to now we considered a particle moving through a stationary fluid and demonstrated that the forces acting on it depend linearly on its velocity. Using Stokes linearity, we can re-phrase this argument – a stationary particle in a flow feels drag and torque as it resists the fluid motion. What is more, the resistance tensor in both cases is one and the same as long as the system is Galilean invariant and the only thing we change is the frame of reference:

$$\begin{pmatrix} F_x \\ F_y \\ T_z \end{pmatrix} = \eta \boldsymbol{R}_{\mathrm{p}} \cdot \begin{pmatrix} u - \dot{x} \\ v - \dot{y} \\ \omega - \dot{\theta} \end{pmatrix}, \quad [5]$$

where the velocity components of the 2D flow field are given by $\boldsymbol{U}_0 = (u, v, \omega)$. However, in confined Stokes flow Galilean invariance is violated (3), which warrants separate resistance tensors for the fluid and the particle:

$$\begin{pmatrix} F_x \\ F_y \\ T_z \end{pmatrix} = \eta \boldsymbol{R}_{\mathrm{f}} \cdot \begin{pmatrix} u \\ v \\ \omega \end{pmatrix} - \eta \boldsymbol{R}_{\mathrm{p}} \cdot \begin{pmatrix} \dot{x} \\ \dot{y} \\ \dot{\theta} \end{pmatrix} \quad [6]$$

The additional resistance the fluid experiences as it flows between the closely spaced confining plates (Fig. 1 *F* in the main text) is incorporated in $\boldsymbol{R}_{\mathrm{f}}$, which results in $\boldsymbol{R}_{\mathrm{f}} \neq \boldsymbol{R}_{\mathrm{p}}$.

In a similar fashion we can incorporate any implicit forces the particle may experience as it moves through the 2D fluid. In the case of confined Stokes flow, additional drag and torque come from the thin liquid gaps separating the particle faces from the confining plates. Physically, these are the forces acting on the faces of the particle as it shears the fluid in the gap. Adding these forces to equation (6) completes the hydrodynamic force balance for a particle in confined Stokes flow:

$$\begin{pmatrix} F_x \\ F_y \\ T_z \end{pmatrix} = \eta \boldsymbol{R}_{\mathrm{f}} \cdot \begin{pmatrix} u \\ v \\ \omega \end{pmatrix} - \eta \boldsymbol{R}'_{\mathrm{p}} \cdot \begin{pmatrix} \dot{x} \\ \dot{y} \\ \dot{\theta} \end{pmatrix} = \begin{pmatrix} 0 \\ 0 \\ 0 \end{pmatrix}, \quad [7]$$

where we have clumped the resistance tensor for the confining wall $\boldsymbol{R}_{\mathrm{w}}$ with $\boldsymbol{R}_{\mathrm{p}}$ into a single particle resistance tensor $\boldsymbol{R}'_{\mathrm{p}} = \boldsymbol{R}_{\mathrm{p}} + \boldsymbol{R}_{\mathrm{w}}$. Solving this system of linear equations yields the force-free velocity $\boldsymbol{U}_{\mathrm{p}}$ of a particle with orientation $\theta$ in a flow with velocity $\boldsymbol{U}_{\mathrm{f}}$. For this equation to hold at different orientations, we need to incorporate the angular dependencies of the resistance tensors, through equation (4). However, it is more straightforward to apply a rotation of $-\Delta\theta$ to the linear velocities of the particle and the flow, rather than a rotation of $\Delta\theta$ to the resistance tensors:

$$\begin{pmatrix} F_x \\ F_y \\ T_z \end{pmatrix} = \eta \boldsymbol{R}_{\mathrm{f}} \cdot \begin{pmatrix} u \cos\theta' + v \sin\theta' \\ -u \sin\theta' + v \cos\theta' \\ \omega \end{pmatrix} - \eta \boldsymbol{R}'_{\mathrm{p}} \cdot \begin{pmatrix} \dot{x} \cos\theta' + \dot{y} \sin\theta' \\ -\dot{x} \sin\theta' + \dot{y} \cos\theta' \\ \dot{\theta} \end{pmatrix} = \begin{pmatrix} 0 \\ 0 \\ 0 \end{pmatrix}, \quad [8]$$

where $\theta' = \theta - \Delta\theta$. As the far field flow is unidirectional, we can set $v$ and $\omega$ to zero:

$$\begin{pmatrix} F_x \\ F_y \\ T_z \end{pmatrix} = \eta \boldsymbol{R}_{\mathrm{f}} \cdot \begin{pmatrix} u \cos\theta \\ -u \sin\theta \\ 0 \end{pmatrix} - \eta \boldsymbol{R}_{\mathrm{p}} \cdot \begin{pmatrix} \dot{x} \cos\theta + \dot{y} \sin\theta \\ -\dot{x} \sin\theta + \dot{y} \cos\theta \\ \dot{\theta} \end{pmatrix} = \begin{pmatrix} 0 \\ 0 \\ 0 \end{pmatrix}, \quad [9]$$

where we have dropped the primes for convenience. Each dot product in equation (9) yields an in-plane force, which needs to be transformed back to the channel frame of reference by rotating it by $\Delta\theta$.

Solving this system yields equations of motion describing both the rotation and drift of a particle with an arbitrary shape in confined Stokes flow (1):

$$\dot{\theta} = \frac{1}{\tau_1} \sin\theta + \frac{1}{\tau_2} \cos\theta \quad [10]$$

$$\frac{\dot{y}}{H} = -\frac{1}{\tau_{y,1}} \sin^2\theta - \frac{1}{\tau_{y,2}} \sin 2\theta + \frac{1}{\tau_{y,3}} \cos^2\theta \quad [11]$$

The generality of these equations, however, comes at the price of overwhelmingly complex expressions for the five timescales $\tau_i$ determining the particle dynamics (equations A.4 through A.10, (1)). This complexity is greatly reduced if one focuses on particles with a certain symmetry.

**C. Resistance tensor and particle symmetry.** For example, objects with a single mirror plane have only two finite timescales, one governing rotation $\tau_1$ and one determining drift $\tau_{y,2}$. These are the two timescales referred to as $\tau$ and $\tau_y$ in the main text. If a particle possesses two mirror planes, such as a rod, its rotational timescale $\tau$ diverges, meaning it does not rotate, but only drifts. Objects with an even higher symmetry, such as cross-like particles or disks, have all their timescales diverging, resulting in fully decoupled modes of motion.

To illustrate these concepts, we present a set of particles with a decreasing number of mirror planes, from 4 to 0 in Fig. S2. Each particle consists of at least one disk and at least one rectangular rod. All particles are oriented at an angle $\theta = 75°$ with respect to the flow $u$ denoted by a black arrow. The angle $\theta$ is defined by two rays starting from the centre of the disk, one parallel to the flow and one parallel to the long axis of the rod. Black dashed lines denote the mirror planes of each particle. The particles are subjected to one and the same confinement, $\tilde{H}_{\mathrm{p}} = H_{\mathrm{p}}/H = 0.80$, and far-field Brinkman flow $\boldsymbol{U}_{\mathrm{f}} = (u, 0, 0)$.

We compute the resistance tensors $\boldsymbol{R}_\mathrm{f}$ and $\boldsymbol{R}_\mathrm{p}$ at $\theta = 75°$ when the particle is moving through an infinitely large domain using a quasi-2D finite element scheme, as detailed by Bet *et al.* (4). We obtain the force- and torque-free velocities of each particle by solving equation (9) numerically. Next, if the particle exhibits any angular velocity, we rotate it clockwise until $\dot{\theta}$ becomes zero, thus obtaining its stable orientation $\theta_\infty = \theta\,(t \to \infty)$, sketched in the second row of Fig. S2. The red arrow and the green arc representing $\dot{y}$ and $\dot{\theta}$ have been enlarged by factors of, respectively, 15 and 5, compared to the blue arrow denoting $\dot{x}$.

While the change in symmetry has little to no effect on $\dot{x}$, it affects the overall particle dynamics drastically through the rotational and drift degrees of freedom. Particles with fewer than two mirror planes exhibit all three modes of motion, which are coupled, as evident from their resistance tensors. Particles possessing two mirror planes have zero angular velocity - their rotation is decoupled from their two translational degrees of freedom. Increasing the symmetry further renders the particle akin to a disk – the particle neither rotates, nor drifts, regardless of its orientation. Furthermore, its resistance tensor is a diagonal matrix, signifying the full decoupling of its degrees of freedom.

A particle's symmetry also affects the number of fixed point orientations it exhibits. While every orientation is stable for objects with two or more mirror planes, particles with a lower symmetry have one stable fixed orientations and an unstable fixed orientation. As discussed in the main text, a particle with a single mirror plane has $\theta_\infty = 0$: its symmetry axis aligns with the flow and its larger building block is upstream. Additionally, this particle exhibits an unstable fixed orientation $\theta^\star_\infty = \pi$, when it aligns to the flow with its larger building block downstream (5). If placed in an unbounded domain or in the centre of a domain bounded by side walls, the particle ceases to drift once $\theta = \theta_\infty$, because the flow disturbances it creates are symmetric about its mirror plane and cancel. However, these flow disturbances are asymmetric when the particle is offset with respect to the centreline of the domain. This asymmetry gives rise to a small lateral velocity, which pushes the particle towards the centreline.

Particles with no mirror planes exhibit a similar long-timescale drift even at very large distances from a side wall. One such particle will retain a constant drift velocity even after it has stopped rotating. Furthermore, unlike symmetric particles which steer away from side walls, a non-symmetric object drifts towards one wall of a channel until it is reflected from it and re-directed towards the other, as shown in Fig. S3 and (1). This type of dynamics, similar to the one observed for rods and symmetric dimers (6, 7), can be traced back to the resistance tensor (cf. Fig. S2, bottom row, columns two and four). The non-zero elements responsible for the translational coupling $\boldsymbol{R}'_{\mathrm{p},12} = \boldsymbol{R}'_{\mathrm{p},21} \neq 0$ in particles with zero and two mirror planes determine their finite drift as they move at $\theta = \theta_\infty \neq 0$. Conversely, particles with a single mirror plane have their translational degrees of freedom decoupled as long as they are not in the vicinity of a wall.

**D. Characteristic timescales $\tau$ and $\tau_y$ for mirror-symmetric particles as functions of particle velocity.** To understand what the two timescales represent for asymmetric disk dimers and mirror symmetric particles in general, we take a look at equations (10) and (11) and set $\tau_2$, $\tau_{y,1}$ and $\tau_{y,3}$ to infinity (1):

$$\dot{\theta} = \tau^{-1} \sin\theta \qquad [12]$$

$$\dot{y}/H = -\tau_y^{-1} \sin 2\theta \qquad [13]$$

Using $\theta$ as detailed in Fig. S1, the rotational timescale is the inverse of the rotational velocity when the particle is perpendicular to the flow. Furthermore, it is always negative as the particle rotates towards an orientation $\theta = 0$. However, as $\tau$ is the intrinsic relaxation time of the process it is natural to define it as a positive number and use a modified version of the equation for rotation (5):

$$\dot{\theta} = -\tau^{-1} \sin\theta \qquad [14]$$

Conversely, the translational time $\tau_y$ is the channel height scaled by the inverse of the drift velocity when the particle is oriented at $\theta = k\pi/2 + \pi/4$ with respect to the flow, where $k$ is an integer (Fig. S1). We gain more insight into $\tau_y$ by considering a well-studied class of mirror-symmetric particles: rods. Recently, Nagel *et al.* (7) derived an expression for the drift velocity of a rod $\dot{y}_\mathrm{rod}$ in confined Stokes flow, relating it to the streamwise velocities $\dot{x}_i$ of the particle:

$$\dot{y}_\mathrm{rod} = \left(\dot{x}_\parallel - \dot{x}_\perp\right) \sin\theta\cos\theta = \frac{\dot{x}_\parallel - \dot{x}_\perp}{2} \sin 2\theta, \qquad [15]$$

where the subscripts $\parallel$ and $\perp$ denote the orientation of the long axis of the rod with respect to the flow. Since the mirror plane of most of the particles we study coincides with their long axis, we use the symmetry plane to define the angle. Substituting equation (15) in the general expression for the drift, equation (13), reveals that $\tau_y$ is a function of $\dot{x}_i$:

$$\tau_y = \frac{2H}{\dot{x}_\perp - \dot{x}_\parallel} \qquad [16]$$

## 2. Obtaining experimental timescales from experimental trajectories of mirror-symmetric particles

The short-timescale dynamics of a particle with at least one mirror plane depends on two characteristic times, $\tau$ and $\tau_y$, as demonstrated in equations 2 and 3 in the main text. Numerically, these timescales can be computed directly from the components of the resistance tensors (1). Alternatively, the timescales also relate to the particle velocities at specific angles: $\tau = -1/\dot{\theta}\,(\theta = \pi/2)$ and $\tau_y = -H/\dot{y}\,(\theta = \pi/4)$. While the former method is experimentally inaccessible, the latter is unreliable as it requires estimating $\tau$ and $\tau_y$ from only two consecutive frames in a time series, recorded with an optical microscope (Fig. S5 *A*).

As each one of these time series contains hundreds of frames, it is preferable to extract $\tau$ and $\tau_y$ from the experimental trajectories via the equations of motion (equations 2 and 3 in main text). We obtain these trajectories from the in-plane coordinates of each building block in a particle. Through trigonometric relations we calculate the orientation of the particle and its centre-of-mass position in each frame Fig. S5 $B$,$C$ and $D$). Thus, we obtain two raw experimental datasets containing $[t, \theta]$ and $[t, y]$, where we have removed any offset due to stage motion or channel tilt.

Instead of attempting to fit the non-linear equations of motion to the raw data, we choose to re-write the equations in a linear form and compute initial guesses for the two timescales through linear fitting. We then feed these guesses to a non-linear minimization function that fits both equations simultaneously, thus avoiding dependence of $\tau_y$ on $\tau$.

We begin by re-writing equation 2 in the main text in linear form:

$$\ln\left(\tan\frac{\theta}{2}\right) = -\frac{t}{\tau_0} + \frac{t_{\perp,0}}{\tau_0} \qquad [17]$$

where $-1/\tau_0$ and $t_{\perp,0}/\tau_0$ are, respectively, the slope and intercept of the fitted line. Estimating $t_{\perp,0} = t\,(\theta = \pi/2)$ directly from the raw data is unreliable due to experimental artefacts such as dust and channel irregularities. These artefacts may temporarily disrupt the rotation of the particle and cause it to rotate more slowly or quickly around $\theta = \pi/2$ without significantly altering the overall trajectory. To prevent such an incorrect offset, we leave $t_{\perp,0}$ as a fitting parameter.

Therefore, we calculate $[t_i, \ln(\tan(\theta_i/2))]$ from $[t_i, \theta_i]$ for each frame $i$ and fit a line to the new dataset (Fig. S5 $E$). Next, we use the slope and intercept from the fit to rescale $[t_i, y_i]$ into a dataset following a linear equation (Fig. S5 $F$):

$$\left[\frac{y_i - y\,(t_{\perp,0})}{2\tau_0 H}, \operatorname{sech}\left(\frac{t_i - t_{\perp,0}}{\tau_0}\right) - 1\right] \qquad [18]$$

We then fit a line with a zero intercept to the new dataset and extract $1/\tau_{y,0}$ as the slope.

Our final step is to construct a cost function $\Sigma_{\text{res}}\,(\tau, \tau_y, t_\perp)$, which minimizes the residuals of the two linear fits simultaneously and takes $\tau_0, \tau_{y,0}$ and $t_{\perp,0}$ as initial conditions (Fig. S5 $G$):

$$\Sigma_{\text{res}}\,(\tau, \tau_y, t_\perp) = \sum_{t_i=1}^{t_{\text{end}}} \left(\frac{t_i - t_\perp}{\tau} + \log\left(\tan\frac{\theta_i}{2}\right)\right)^2 + \sum_{t_i=1}^{t_{\text{end}}} \left(1 - \operatorname{sech}\left(\frac{t_i - t_\perp}{\tau}\right) + \tau_y \frac{y_i - y\,(t_\perp)}{2\tau H}\right)^2 \qquad [19]$$

The output of the cost function $(\tau_{\text{exp}}, \tau_{\text{y,exp}}, t_\perp)$ is used to rescale the experimental data and collapse it onto equations 2 and 3 in the main text (Fig. S5 $H$). We apply this procedure to all experimental time series we report in the following section.

## 3. Settings for the finite element solver

We start building up the 3D geometry with a cuboid with dimensions height $\times$ width $\times$ length $= H\times \sim 16H\times \sim 32H$ representing the fluid domain. Within it, we compose a particle from cylinders or square/triangular prisms connected with cuboids. All building blocks have rounded edges and are joined through a Boolean union. This results in a particle surface containing a multitude of two-dimensional domains separated by non-physical boundaries. To relax and improve meshing, we merge these domains in such a way that the final geometry contains only three surfaces: a top wall facing the confining channel wall, a side wall surrounded by the flowing fluid and a curved edge connecting them. Next, we cut the particle out from the fluid domain through a Boolean difference. We exploit the symmetry present along the channel height by subtracting a thinner cuboid with dimensions $H/2\times \sim 16H\times \sim 32H$ from the fluid domain.

We set an inflow velocity of $u$ on one of the walls normal to $x$ and a zero pressure boundary condition on the other. We apply no slip boundary conditions to the two walls normal to $y$ and to the top wall of the channel. The lower wall of the domain, now representing the channel centre plane, is converted to a symmetry boundary. The boundaries created by removing the particle from the domain are defined as no-slip moving walls with velocities $\left(\dot{x} - \dot{\theta}\,(y - c_{0,y})\,, \dot{y} + \dot{\theta}\,(x - c_{0,x})\,, 0\right)$, where $x$ and $y$ are the coordinates of the wall element and $(c_{0,x}, c_{0,y}) = \boldsymbol{c}_0$ are the components of the particle centre of mass.

To test how these geometry optimizations affect our results, we gradually optimize the geometry of a model particle, compute the timescales $\tau$ and $\tau_y$ in each case and compare them in Fig. S16. As a base case we use a disk trimer with $\kappa = 1.5$ and $\phi = 90°$ with straight edges, where we do not exploit symmetry and do not merge faces. While both techniques have barely any effect on the timescales, using symmetry boundary conditions reduces both the execution time and the memory required (Fig. S16 $D$ and $E$). Making the particle edges round has a noticeable effect on the timescales, which we investigate in Fig. S17. By gradually increasing the radius of curvature relative to the channel height, we observe a decrease in the timescales, which, however becomes less pronounced as we increase the mesh fineness. In light of these observations we conclude that the proposed optimization techniques have no significant effect on the computational results. We use a predefined Fine mesh on the particle surfaces and a predefined Coarse mesh everywhere else, both calibrated for fluid dynamics.

We solve the set of governing equations using the MUMPS direct solver (8, 9) through a single-level mesh refinement scheme. In short, we first compute a solution on the initial mesh, estimate the global error in the solution using the $L^2$ norm of the error and locally refine the initial mesh towards a rough global error minimum. To keep the memory required for the computation under 64 GB, we permit the number of mesh elements to, at most, double. We also prevent excessive mesh coarsening by setting the maximum coarsening factor to 1.5. We opt for a single level of mesh refinement, as consecutive refinement cycles do not decrease the global error any further, yet require more time and memory (10).

We obtain the trajectory of a particle through a first order time integration scheme, where we apply $\left(\dot{x}, \dot{y}, \dot{\theta}\right)$ over a timestep $t_{\text{step}}$. Every iteration, we determine $t_{\text{step}}$ as the smallest of three values: 5, $\tau/10$ or the minimum distance between the particle and the closest side wall divided by $10\dot{y}$. This method ensures shorter timesteps for particles approaching the side wall of a channel and prevents large timesteps for slowly rotating or non-rotating particles far from walls. After determined $t_{\text{step}}$, the particle is rotated about its centre of mass by $\dot{\theta} t_{\text{step}}$ and then displaced along the transversal direction by $\dot{y} t_{\text{step}}$, while its longitudinal displacement is stored for post-processing. We move the particle only along $y$ to avoid unnecessary re-meshing and minimize domain size influences.

## 4. Minimalistic scaling relations for rotational timescale $\tau$ and translational timescale $\tau_y$

Modelling the drift timescale $\tau_y = 2H/\left(\dot{x}_\perp - \dot{x}_\parallel\right)$ requires estimating the two streamwise velocities $\dot{x}_\perp$ and $\dot{x}_\parallel$ when the particle is, respectively, perpendicular $\theta = \pi/2$ and parallel $\theta = 0$ to the flow (SI Text 1D). We obtain $\dot{x}_\perp$ and $\dot{x}_\parallel$ by balancing the pressure force exerted by the flow on the particle sides to the viscous drag from the confining walls acting on the particle faces. We then re-use the expression for the pressure force acting on a particle oriented normal to the flow to compute the rotational timescale.

The streamwise drag force from the confining walls of the channel is (4):

$$F_{\text{w}} = -\frac{2\eta}{h}\int_{S_{\text{p}}} \mathrm{d}S\left(\dot{x} + \dot{\theta}\times(\boldsymbol{r} - \boldsymbol{c}_0)\right), \qquad [20]$$

where $\eta$ is the fluid viscosity, $h$ is the the thickness of the fluid layer separating the particle from the confining wall and $S_{\text{p}}$ is the area of the particle face.The distance from any differential area $\mathrm{d}S$ to an arbitrary reference point is $\boldsymbol{r}$ and $\boldsymbol{c}_0$ is the distance from the particle centroid to the reference point. When the particle is parallel to the flow, the second term in equation (20) drops, because $\dot{\theta} = 0$. We also neglect it when the particle is perpendicular to the flow due to the weak coupling between streamwise motion and rotation. This weak coupling is reflected by the components of the resistance tensor as $R_{11} \gg R_{13}$. Therefore, the wall force acting on the faces of the particle is:

$$F_{\text{w},i} = -\frac{2\eta}{h}\dot{x}_i S_{\text{p}}, \qquad [21]$$

where the subscript $i$ in both the force and the velocity denotes particle orientation.

We balance $F_{\text{w},i}$ to the hydrodynamic force exerted by the flow on the particle sides $F_{\text{f},i}$. This flow force emerges due to two effects: fluid pressure and viscous drag. In confined Stokes flow their ratio scales as $F_{\text{visc}}/F_{\text{press}} \sim (H/R)^2$, where $R$ is a particle length scale, namely, the radius for circular particles (11). We choose $R = L_i/2$ for the rod-like dimers and trimers under consideration. While the pressure force dominates over the viscous force when our particles are oriented normal to the flow $(2H/L_\perp)^2 \lesssim 4$, the force ratio is close to unity when they are aligned with it. Nevertheless, we neglect the viscous contribution to $F_{\text{f},i}$ and bear in mind that this ultimately leads to an underestimation of $\tau_y$.

The force pushing the particle forward scales with the height of the particle $H_{\text{p}}$, its length normal to the flow $L_i$ and the local pressure disturbance $\Delta p(x,y)$: $F_{\text{f},i} \simeq -H_{\text{p}} L_i \Delta p(x,y)$. While the former two parameters are readily available experimentally, the pressure disturbance requires some assumptions. Generally, $\Delta p(x,y)$ scales with the far-field pressure gradient $\nabla p = -12\eta u/H^2$ and the local width of the particle $\Delta x(y)$ (11). In other words, the further the particle protrudes away from its mirror plane, the stronger the disturbance it creates. Instead of using the local width, we propose a geometrically averaged width $\sqrt{S_{\text{p}}/\pi} \times L_\parallel/L_\perp$, where we compute an equivalent particle radius through particle area and scale it with the aspect ratio. Filling in the geometrically averaged width in the scaling expression for $F_{\text{f},i}$ yields:

$$F_{\text{f},i} \simeq 12\eta\frac{u}{H^2}H_{\text{p}}L_\parallel\sqrt{\frac{S}{\pi}} \times \frac{L_i}{L_\perp} \qquad [22]$$

Balancing the drag $F_{\text{w},i}$ and pressure $F_{\text{f},i}$ forces yields the streamwise velocity:

$$\dot{x}_i \simeq \frac{6h}{H} \times \frac{u}{H} \times \frac{H_{\text{p}}}{\sqrt{\pi S_{\text{p}}}}\frac{L_\parallel}{L_\perp}L_i \qquad [23]$$

With $\tilde{h} = h/H$, the drift timescale is then:

$$\tau_{y,\text{scaling}} \simeq 2H \times \frac{1}{6\tilde{h}H_{\text{p}}} \times \frac{H}{u} \times \frac{\sqrt{\pi S_{\text{p}}}}{L_\perp - L_\parallel}\frac{L_\perp}{L_\parallel} \qquad [24]$$

Next, we turn our attention to the rotational timescale $\tau = -1/\dot{\theta}\,(\theta = \pi/2)$. We estimate the rotational velocity in a manner similar to the one used for $x_i$ – we balance the torque the flow supplies to the particle sides with the Couette torque from the confining walls: $T_{\text{f}} + T_{\text{w}} = 0$. We link the wall torque to the polar moment of inertia of the particle. We express the fluid torque as the fluid force $F_{\text{f},\perp}$ acting on an arm, whose magnitude depends on the particle asymmetry.

The wall torque, when the particle is perpendicular to the flow, is (4):

$$T_{\text{w}} = -\frac{2\eta}{h}\int_{S_{\text{p}}} \mathrm{d}S\left((\boldsymbol{r} - \boldsymbol{c}_0) \times \left((\dot{x}, \dot{y}) + \dot{\theta}\times(\boldsymbol{r} - \boldsymbol{c}_0)\right)\right), \qquad [25]$$

The linear velocity term drops from the expression because the average weighted distance of every $\mathrm{d}S$ from the centroid is zero:

$$\boldsymbol{c}_0 = \frac{\int_{S_\mathrm{p}} \boldsymbol{r}\mathrm{d}S}{\int_{S_\mathrm{p}} \mathrm{d}S} \tag{26}$$

The wall torque is then simplified to:

$$T_\mathrm{w} = -\frac{2\eta}{h}\dot{\theta}\int_{S_\mathrm{p}} (\boldsymbol{r}-\boldsymbol{c}_0)^2 \,\mathrm{d}S = -\frac{2\eta}{h}\dot{\theta}I_\mathrm{p}, \tag{27}$$

where we substitute the second moment of the area with the polar moment of inertia $I_\mathrm{p}$.

We once again assume that the motion of the particle is dominated by pressure forces. Then, the torque due to flow is:

$$T_\mathrm{f} = \int_{P_\mathrm{p}} \mathrm{d}P_\mathrm{p} F_{\mathrm{f},\perp}(x,y) \times (\boldsymbol{r}-\boldsymbol{c}_0), \tag{28}$$

where we integrate along the perimeter $P_\mathrm{p}$ of the particle. To re-use the expression for $F_{\mathrm{f},\perp}$ in this context, we propose to implicitly integrate along the perimeter, by substituting $\boldsymbol{r}-\boldsymbol{c}_0$ with $r_\mathrm{arm} = |\boldsymbol{c}_\mathrm{p}-\boldsymbol{c}_0|$. The point $\boldsymbol{c}_\mathrm{p}$ is the center of perimeter and lies on the mirror plane. If we draw a line normal to the mirror plane through $\boldsymbol{c}_\mathrm{p}$ it will split the particle in two pieces with equal perimeter. Thus, we propose the following expression for the torque due to flow:

$$T_\mathrm{f} \simeq 12\eta\frac{u}{H^2}H_\mathrm{p}L_\parallel\sqrt{\frac{S}{\pi}} \times r_\mathrm{arm} \tag{29}$$

Adding $T_\mathrm{f}$ to $T_\mathrm{w}$ and isolating the inverse of the rotational velocity yields:

$$\tau_\mathrm{scaling} \simeq \frac{1}{6\tilde{h}H_\mathrm{p}} \times \frac{H}{u} \times \frac{\sqrt{\pi}I_\mathrm{p}}{r_\mathrm{arm}L_\parallel\sqrt{S_\mathrm{p}}} \tag{30}$$

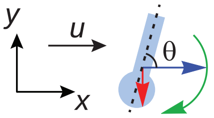


$$R_p = 177 \times \begin{pmatrix} 1 & -0.13 & -0.14 \\ -0.13 & 0.56 & 0.04 \\ -0.14 & 0.04 & 0.46 \end{pmatrix}$$

**Fig. S1. Resistance tensor of a 2D particle with a single mirror plane.** The particle is oriented at an angle $\theta = 75°$ with respect to the flow $u$ denoted by a black arrow. The angle $\theta$ is defined by two rays starting from the centre of the disk, one parallel to $u$ and one parallel to the mirror plane of the particle (dashed black line). Such a particle exhibits three modes of motion: longitudinal and transversal translation along $(x, y)$ and in-plane rotation $\dot{\theta}$ depicted by blue, red and green arrows, respectively. These degrees of freedom are coupled with each other as reflected by the non-zero components in the particle's resistance tensor $R_{\mathrm{p}}$. We visualize this coupling by colour coding the resistance tensor – the two colours of the off-diagonal elements correspond to the colours of the coupled degrees of freedom.

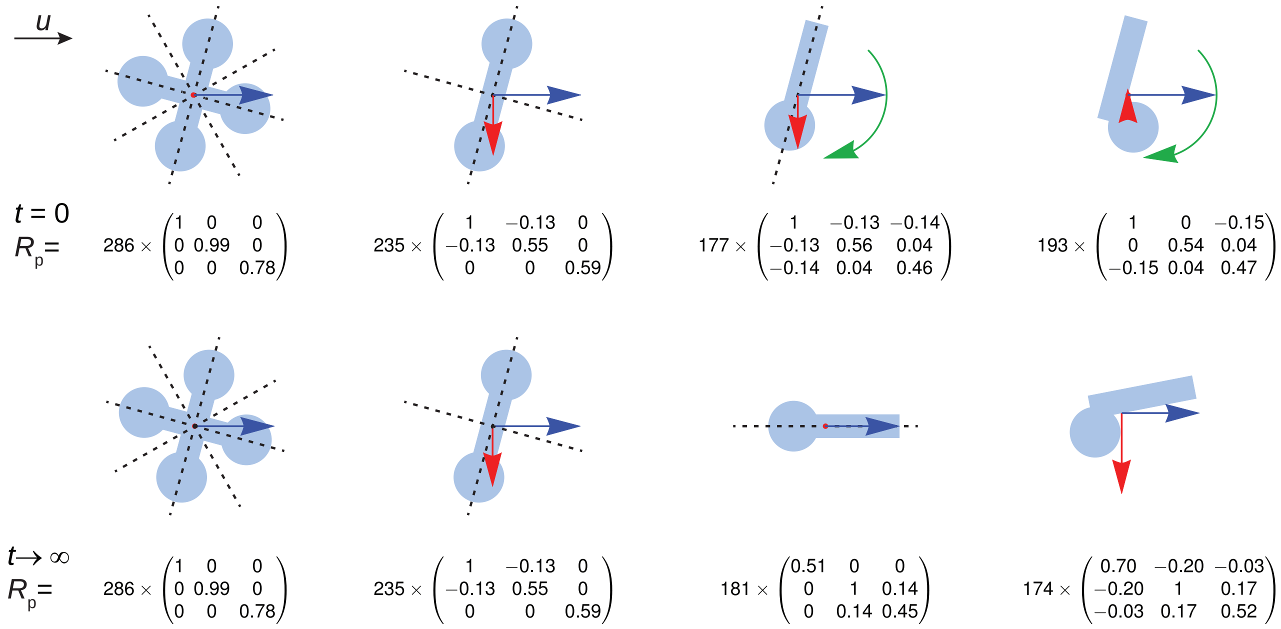


**Fig. S2. The resistance tensor as a function of particle symmetry and orientation.** Far from side walls, particles having more than one mirror plane do not rotate, regardless of their orientation, evident from the zero elements of their coupling tensors (columns one and two). Conversely, particles with one mirror plane rotate until they acquire a stable orientation at which their streamwise translation is decoupled from their cross-stream motion and rotation (column three). Reducing the symmetry even further results in a particle that rotates, yet has a finite cross-stream velocity even after acquiring a stable orientation (column four).

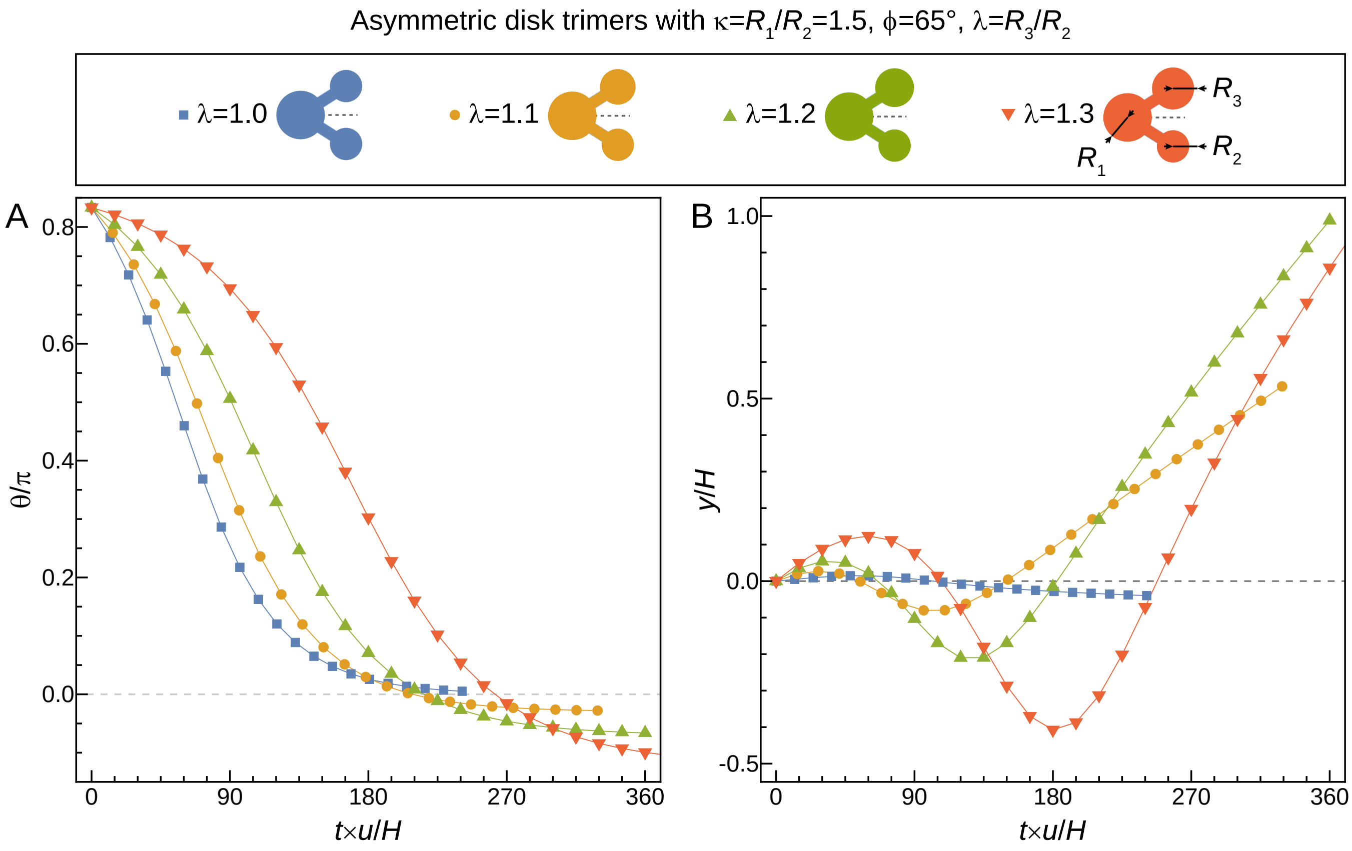


**Fig. S3. Long-timescale drift of particles without mirror planes.** (*A*) While a mirror symmetric particle aligns with the flow (blue squares), disk trimers acquire a non-zero stable fixed orientation $\theta_\infty$. This fixed orientation $\theta_\infty$ is defined with respect to the bisector (dashed grey line) of the angle between the two 'legs', $\phi$. (*B*) After ceasing to rotate, mirror symmetric particles experience a negligible drift towards the centreline of the channel, dictated by its finite width. In contrast, asymmetric particles moving at $\theta_\infty$ create asymmetric flow disturbances and exhibit a steady drift towards the side wall of the channel.

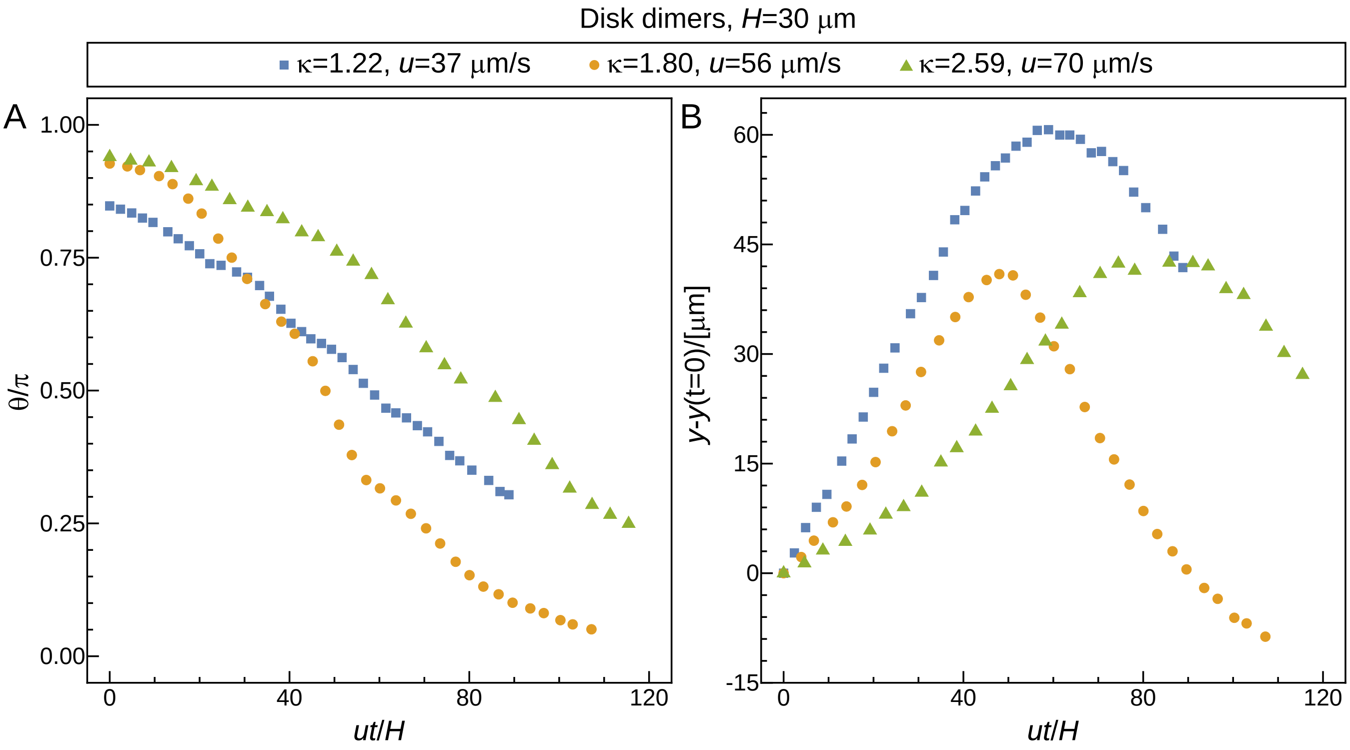


**Fig. S4. Raw experimental trajectories of disk dimers.** Different disk dimers rotate with different velocities (*A*) and follow different in-plane trajectories (*B*). Real time $t$ is rescaled with the channel height $H$ and the far-field flow velocity $u$ to account for different experimental conditions. The flow velocity $u$ is measured by tracking fluorescent microspheres.

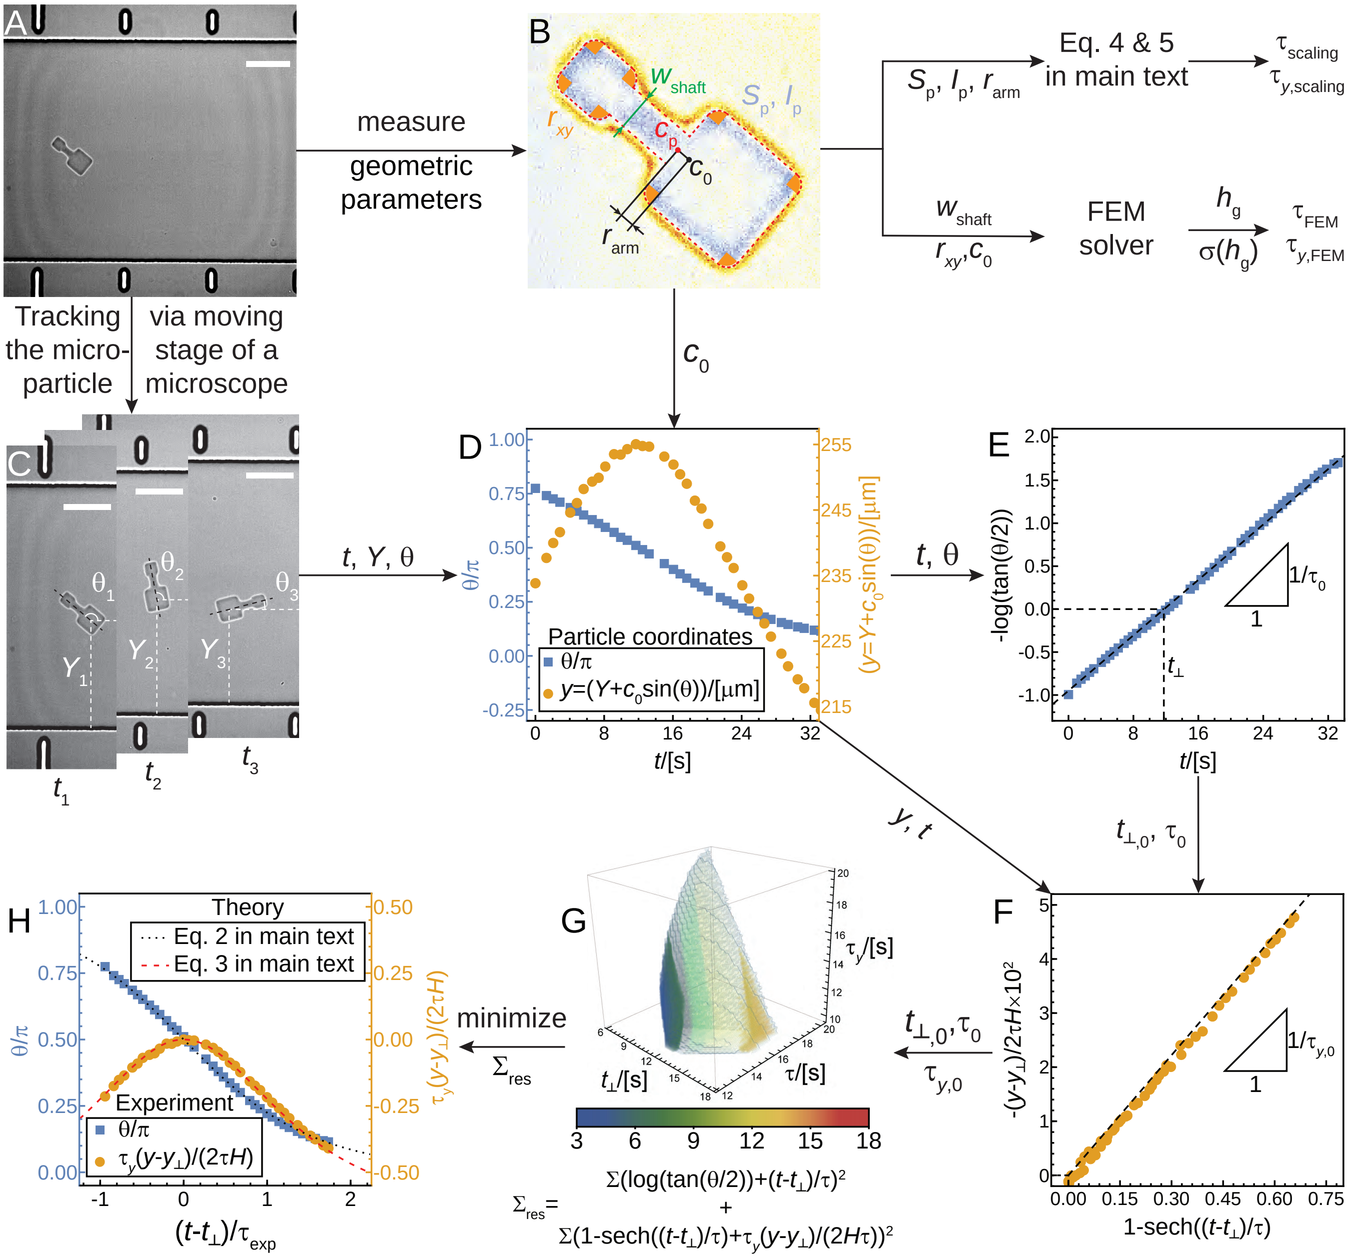


**Fig. S5. Numerical procedure to obtain experimental timescales.** (*A*) A particle, produced through stop-flow lithography, is set it in motion by supplying a pressure drop across the channel. We track its motion via optical microscopy and keep it within the field of view by moving the microscope stage in a stepwise manner. (*B*) Comparing experimental timescales to finite element computations and testing the accuracy of equations 4 and 5 in the main text requires measuring the particle's geometric parameters. These particle parameters include, but are not limited to, the area $S_\mathrm{p}$, area moment of inertia $I_\mathrm{p}$, in-plane radius of curvature $r_{xy}$ and position of the centroid relative to the centre of the building block $c_0$. (*C*) Through image processing techniques, we obtain the coordinates of the particle building blocks and compute $\theta_i$ at each time instant $t_i$. (*D*) We compute the centre-of-mass coordinates of the particle from its orientation, $c_0$ and the lateral position of its large building block. (*E*-*F*) Linear fitting of equations (17) and (18) results in initial guesses for $\tau$, $\tau_y$ and $t_\perp$. (*G*) A cost function $\Sigma_\mathrm{res}$, minimizing the sum of residuals for both equation, yields optimal values for the timescales. (*H*) Scaled experimental time, orientation and lateral position show very good agreement with equations 2 and 3 in the main text. Scale bars are $100\,\mu\mathrm{m}$.

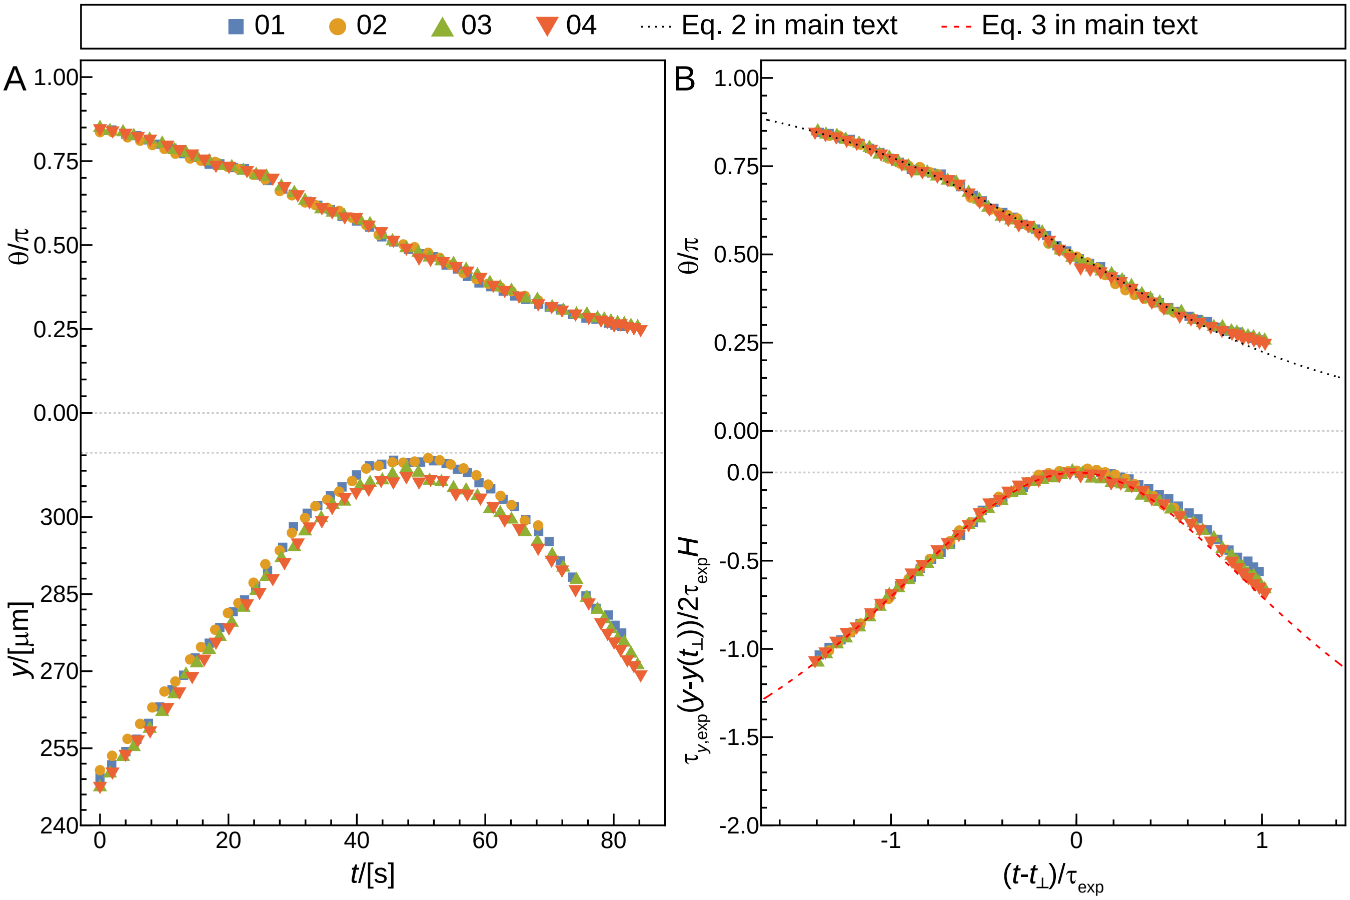


**Fig. S6. Raw and scaled experimental trajectories for a disk dimer with $\kappa = 1.22$** (*A*) Orientation of the particle with respect to the flow (top) and its dimensional transversal position (bottom) as functions of real time. The transversal velocity of the particle changes sign at $\theta \approx \pi/2$. (*B*) Particle orientation (top) and scaled transversal position (bottom) as functions of scaled time. Both the rotation and translation of the particle are described well by equations 2 and 3 in the main text. Different experimental datasets are denoted by different numbers in the figure legend. In all cases the experimental uncertainty is smaller than the symbol size. The timescales used to re-scale each experimental dataset are given the Table S1.

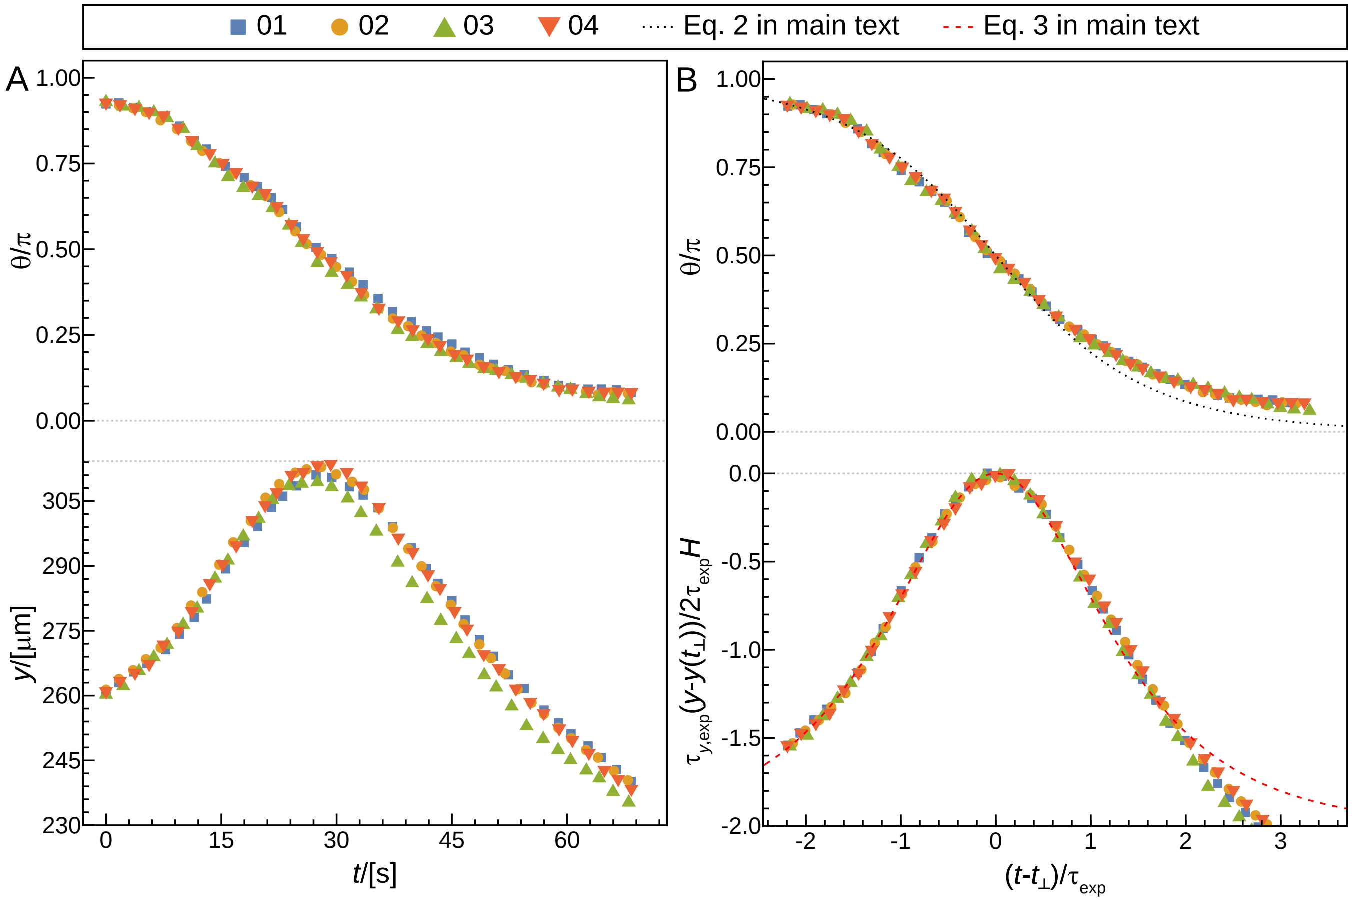


**Fig. S7. Raw and scaled experimental trajectories for a disk dimer with** $\kappa = 1.54$ (*A*) Orientation of the particle with respect to the flow (top) and its dimensional transversal position (bottom) as functions of real time. The transversal velocity of the particle changes sign at $\theta \approx \pi/2$. (*B*) Particle orientation (top) and scaled transversal position (bottom) as functions of scaled time. Both the rotation and translation of the particle are described well by equations 2 and 3 in the main text. Different experimental datasets are denoted by different numbers in the figure legend. In all cases the experimental uncertainty is smaller than the symbol size. The timescales used to re-scale each experimental dataset are given the Table S1.

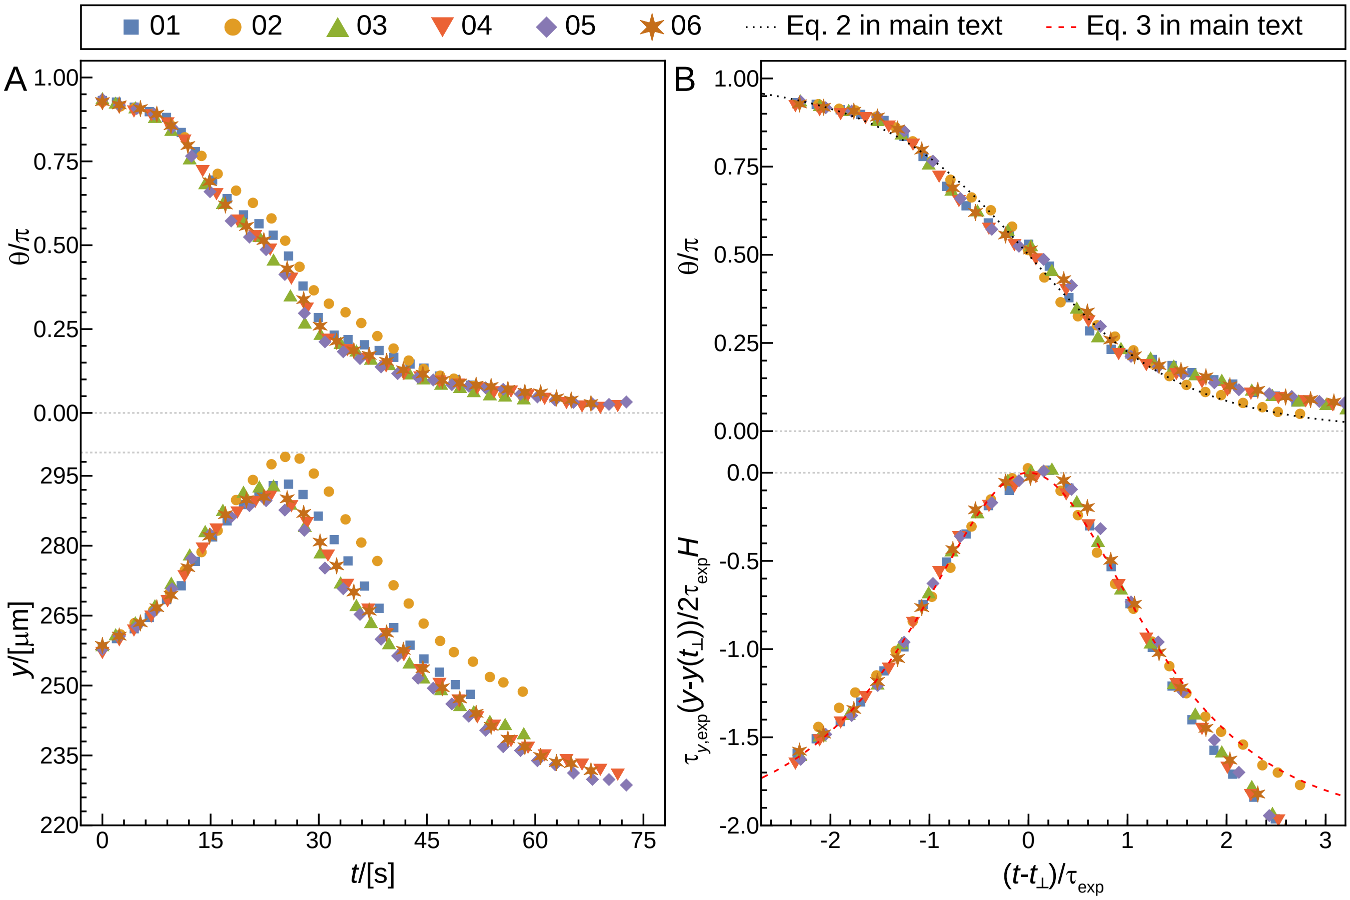


**Fig. S8. Raw and scaled experimental trajectories for a disk dimer with** $\kappa = 1.80$ (*A*) Orientation of the particle with respect to the flow (top) and its dimensional transversal position (bottom) as functions of real time. The transversal velocity of the particle changes sign at $\theta \approx \pi/2$. (*B*) Particle orientation (top) and scaled transversal position (bottom) as functions of scaled time. Both the rotation and translation of the particle are described well by equations 2 and 3 in the main text. Different experimental datasets are denoted by different numbers in the figure legend. In all cases the experimental uncertainty is smaller than the symbol size. The timescales used to re-scale each experimental dataset are given the Table S1.

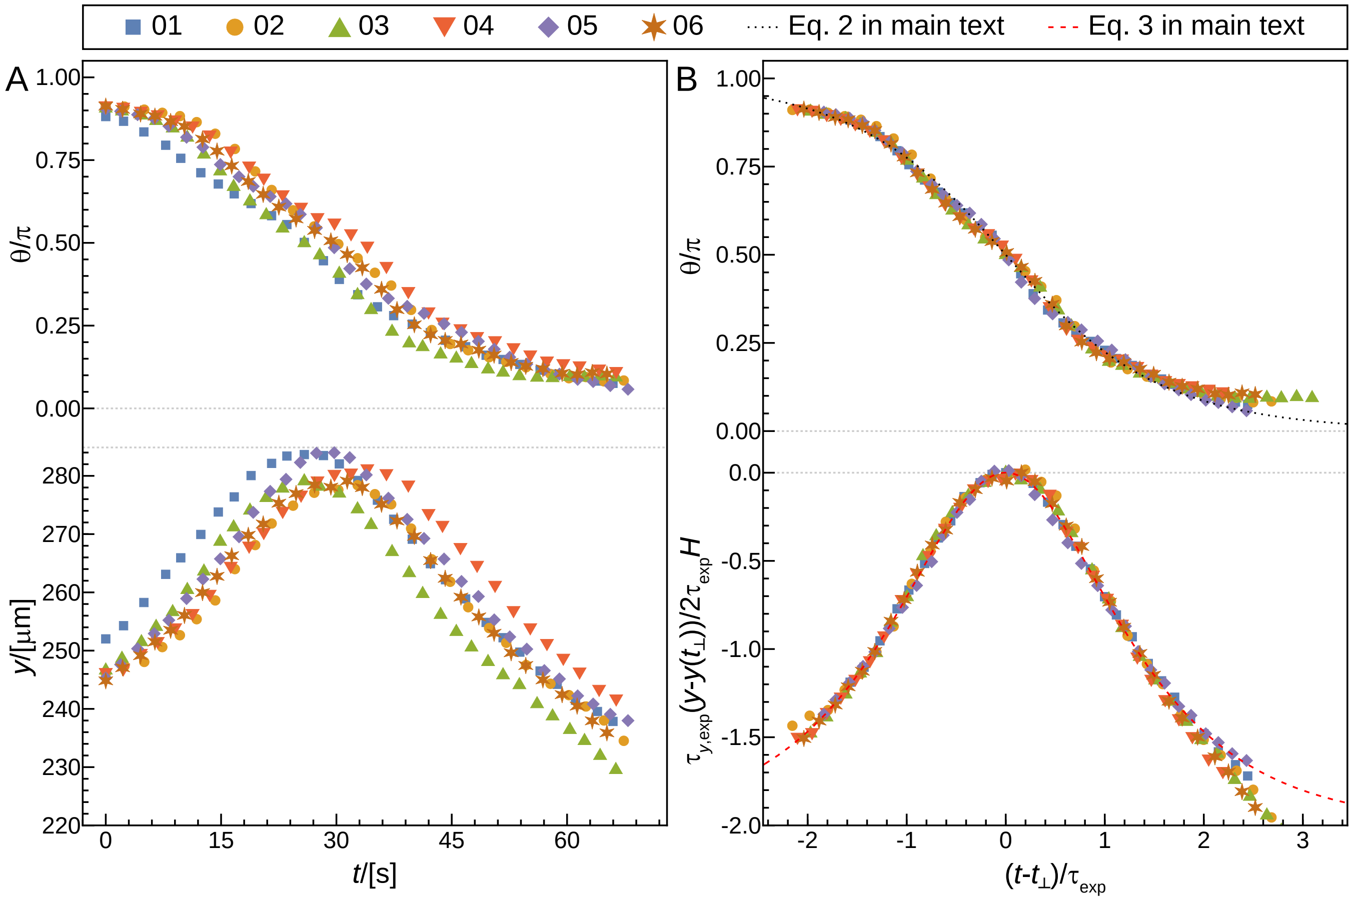


**Fig. S9. Raw and scaled experimental trajectories for a disk dimer with** $\kappa = 2.04$ (*A*) Orientation of the particle with respect to the flow (top) and its dimensional transversal position (bottom) as functions of real time. The transversal velocity of the particle changes sign at $\theta \approx \pi/2$. (*B*) Particle orientation (top) and scaled transversal position (bottom) as functions of scaled time. Both the rotation and translation of the particle are described well by equations 2 and 3 in the main text. Different experimental datasets are denoted by different numbers in the figure legend. In all cases the experimental uncertainty is smaller than the symbol size. The timescales used to re-scale each experimental dataset are given the Table S1.

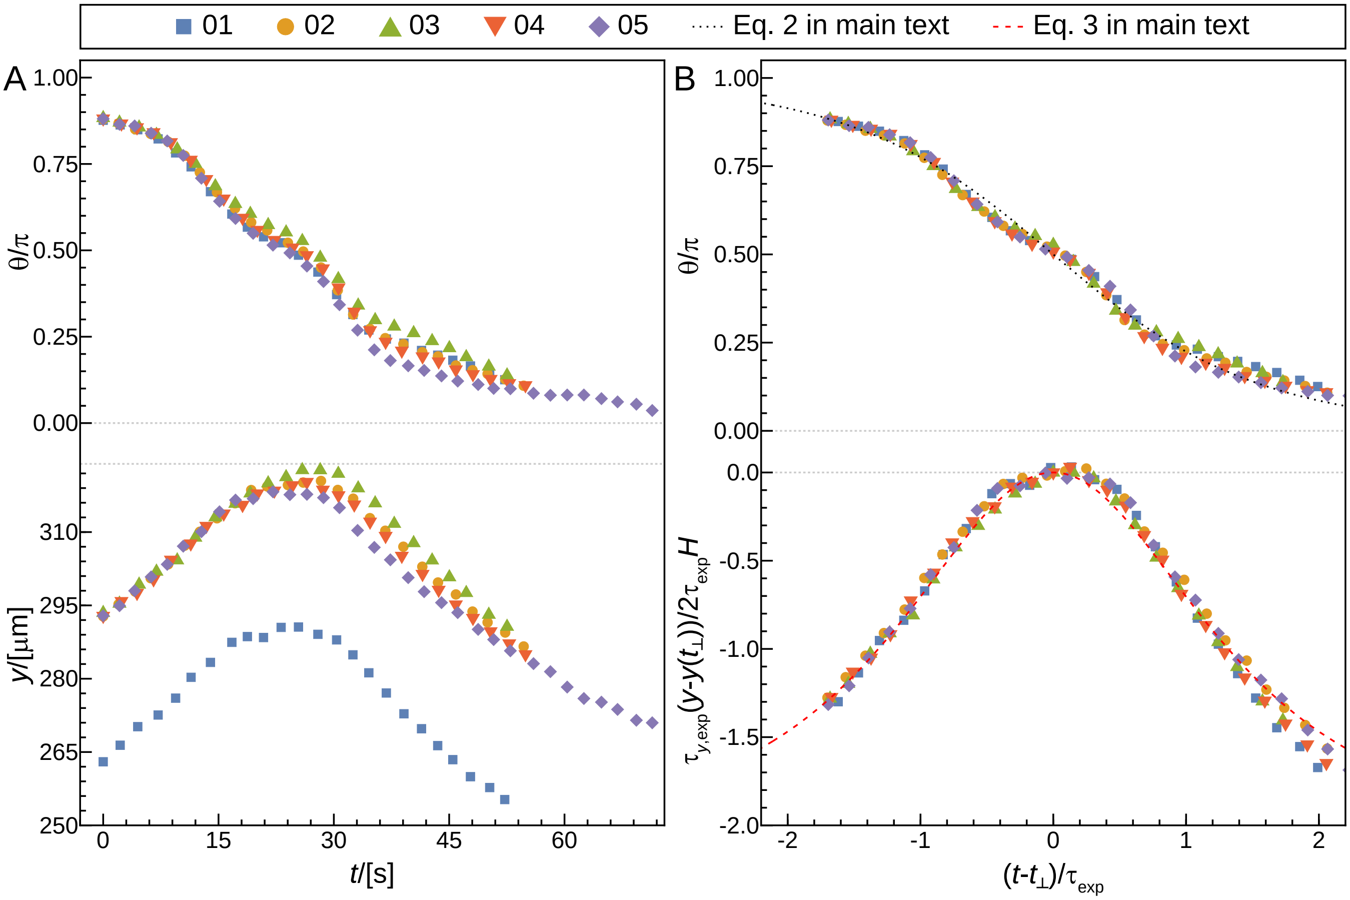


**Fig. S10. Raw and scaled experimental trajectories for a disk dimer with** $\kappa = 2.29$ (*A*) Orientation of the particle with respect to the flow (top) and its dimensional transversal position (bottom) as functions of real time. The transversal velocity of the particle changes sign at $\theta \approx \pi/2$. (*B*) Particle orientation (top) and scaled transversal position (bottom) as functions of scaled time. Both the rotation and translation of the particle are described well by equations 2 and 3 in the main text. Different experimental datasets are denoted by different numbers in the figure legend. In all cases the experimental uncertainty is smaller than the symbol size. The timescales used to re-scale each experimental dataset are given the Table S1.

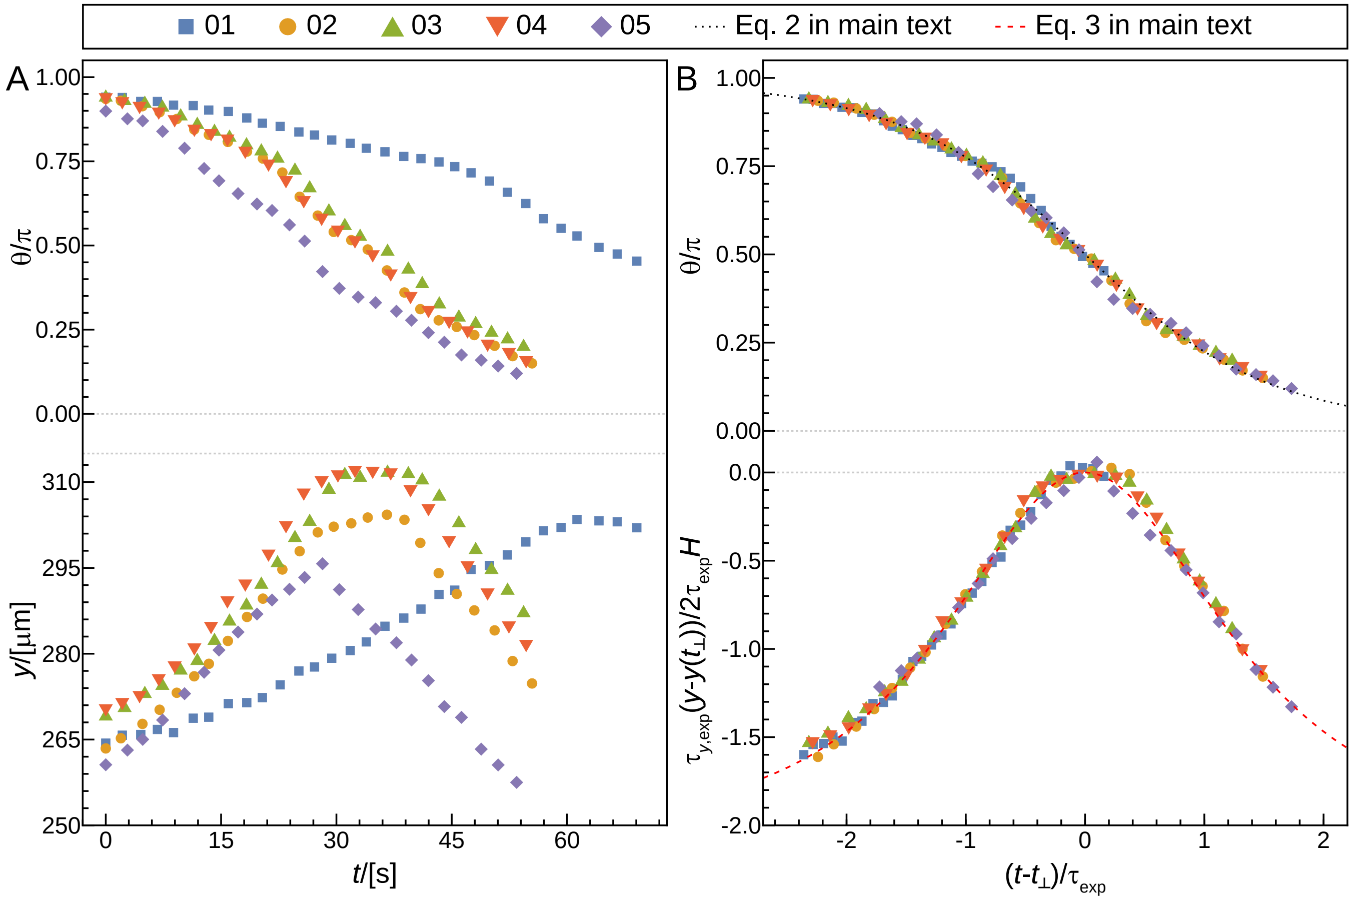


**Fig. S11. Raw and scaled experimental trajectories for a disk dimer with** $\kappa = 2.59$ (*A*) Orientation of the particle with respect to the flow (top) and its dimensional transversal position (bottom) as functions of real time. The transversal velocity of the particle changes sign at $\theta \approx \pi/2$. (*B*) Particle orientation (top) and scaled transversal position (bottom) as functions of scaled time. Both the rotation and translation of the particle are described well by equations 2 and 3 in the main text. Different experimental datasets are denoted by different numbers in the figure legend. In all cases the experimental uncertainty is smaller than the symbol size. The timescales used to re-scale each experimental dataset are given the Table S1.

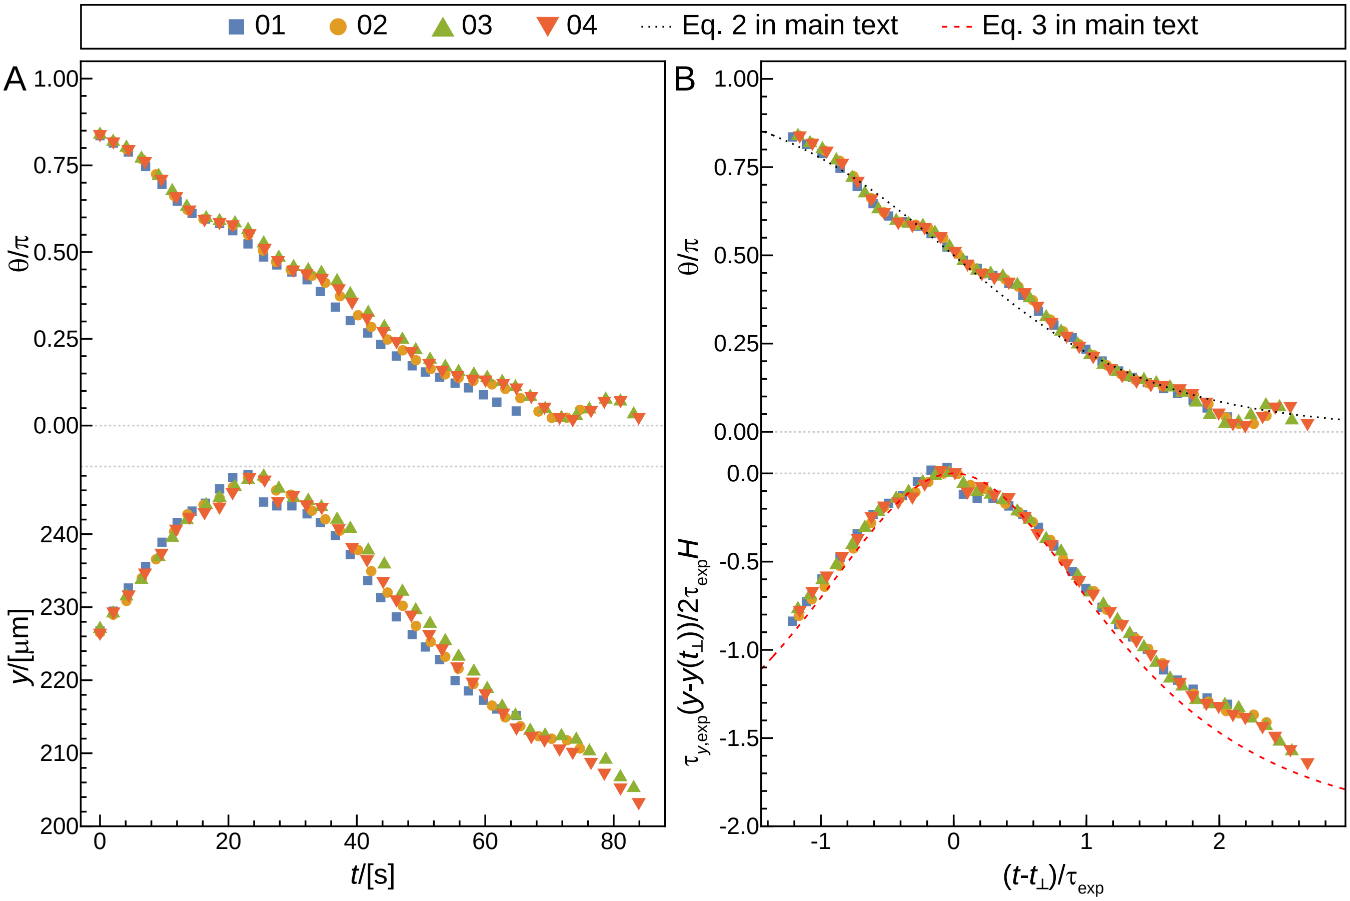


**Fig. S12. Raw and scaled experimental trajectories for a triangular dimer with** $\kappa = 2.92$ (*A*) Orientation of the particle with respect to the flow (top) and its dimensional transversal position (bottom) as functions of real time. The transversal velocity of the particle changes sign at $\theta \approx \pi/2$. (*B*) Particle orientation (top) and scaled transversal position (bottom) as functions of scaled time. Both the rotation and translation of the particle are described well by equations 2 and 3 in the main text. Different experimental datasets are denoted by different numbers in the figure legend. In all cases the experimental uncertainty is smaller than the symbol size. The timescales used to re-scale each experimental dataset are given the Table S1.

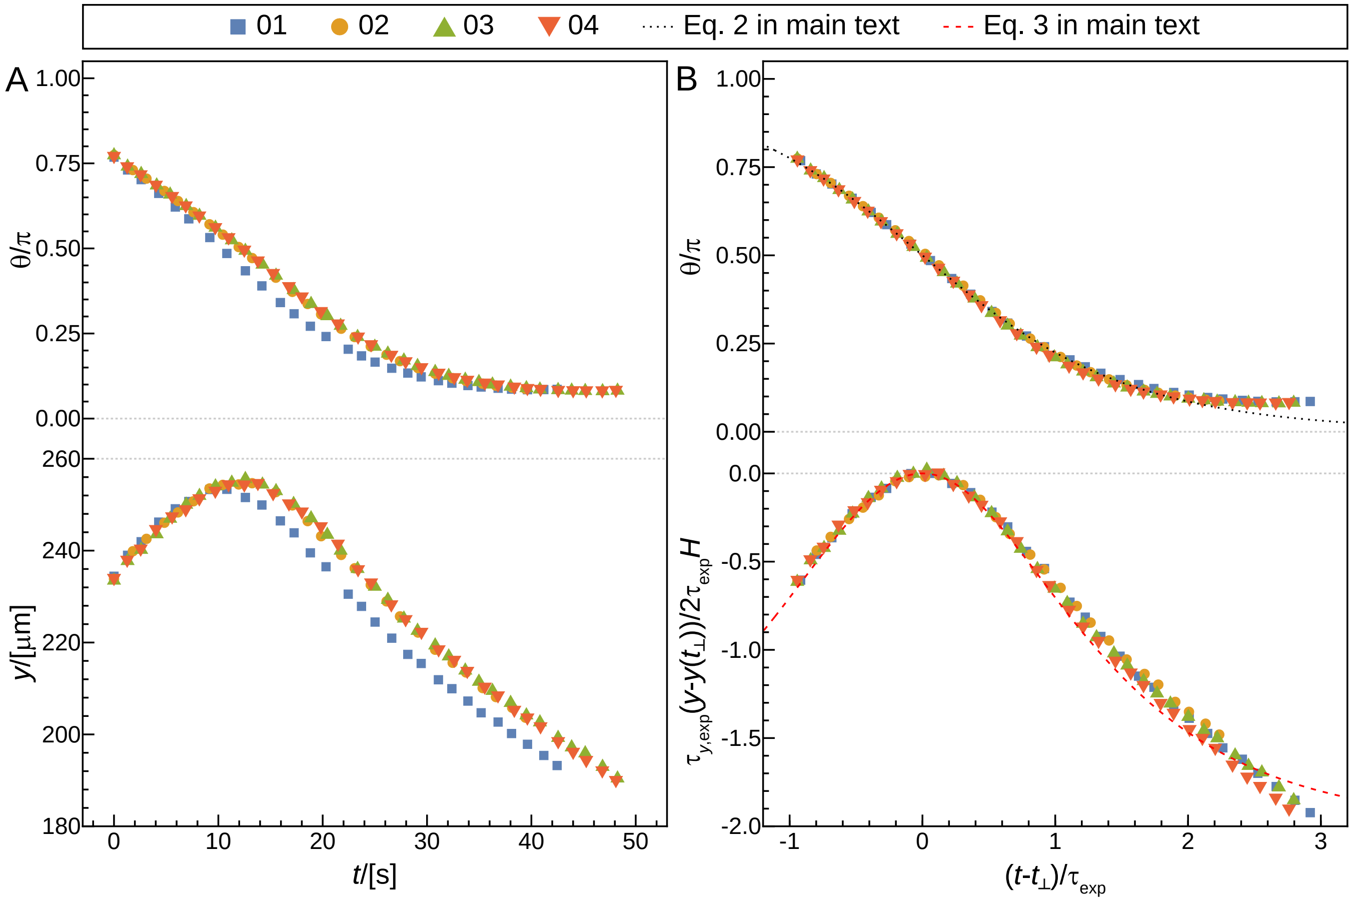


**Fig. S13. Raw and scaled experimental trajectories for a square dimer with** $\kappa = 1.85$ (*A*) Orientation of the particle with respect to the flow (top) and its dimensional transversal position (bottom) as functions of real time. The transversal velocity of the particle changes sign at $\theta \approx \pi/2$. (*B*) Particle orientation (top) and scaled transversal position (bottom) as functions of scaled time. Both the rotation and translation of the particle are described well by equations 2 and 3 in the main text. Different experimental datasets are denoted by different numbers in the figure legend. In all cases the experimental uncertainty is smaller than the symbol size. The timescales used to re-scale each experimental dataset are given the Table S1.

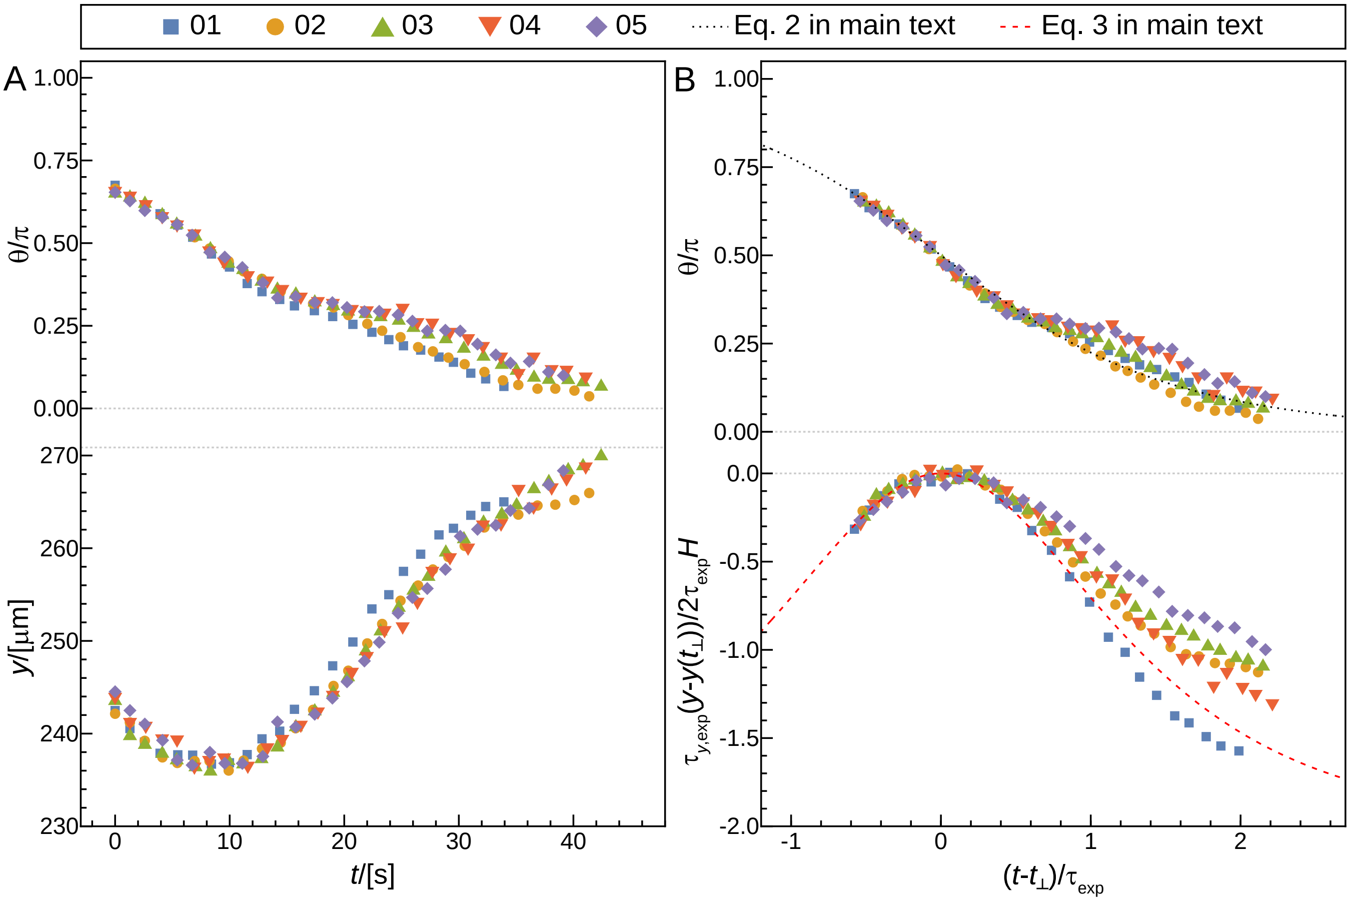


**Fig. S14. Raw and scaled experimental trajectories for a disk trimer with** $\kappa = 1.54$, $\phi = 90°$ (*A*) Orientation of the particle with respect to the flow (top) and its dimensional transversal position (bottom) as functions of real time. The transversal velocity of the particle changes sign at $\theta \approx \pi/2$. (*B*) Particle orientation (top) and scaled transversal position (bottom) as functions of scaled time. Both the rotation and translation of the particle are described well by equations 2 and 3 in the main text. Different experimental datasets are denoted by different numbers in the figure legend. In all cases the experimental uncertainty is smaller than the symbol size. The timescales used to re-scale each experimental dataset are given the Table S1.

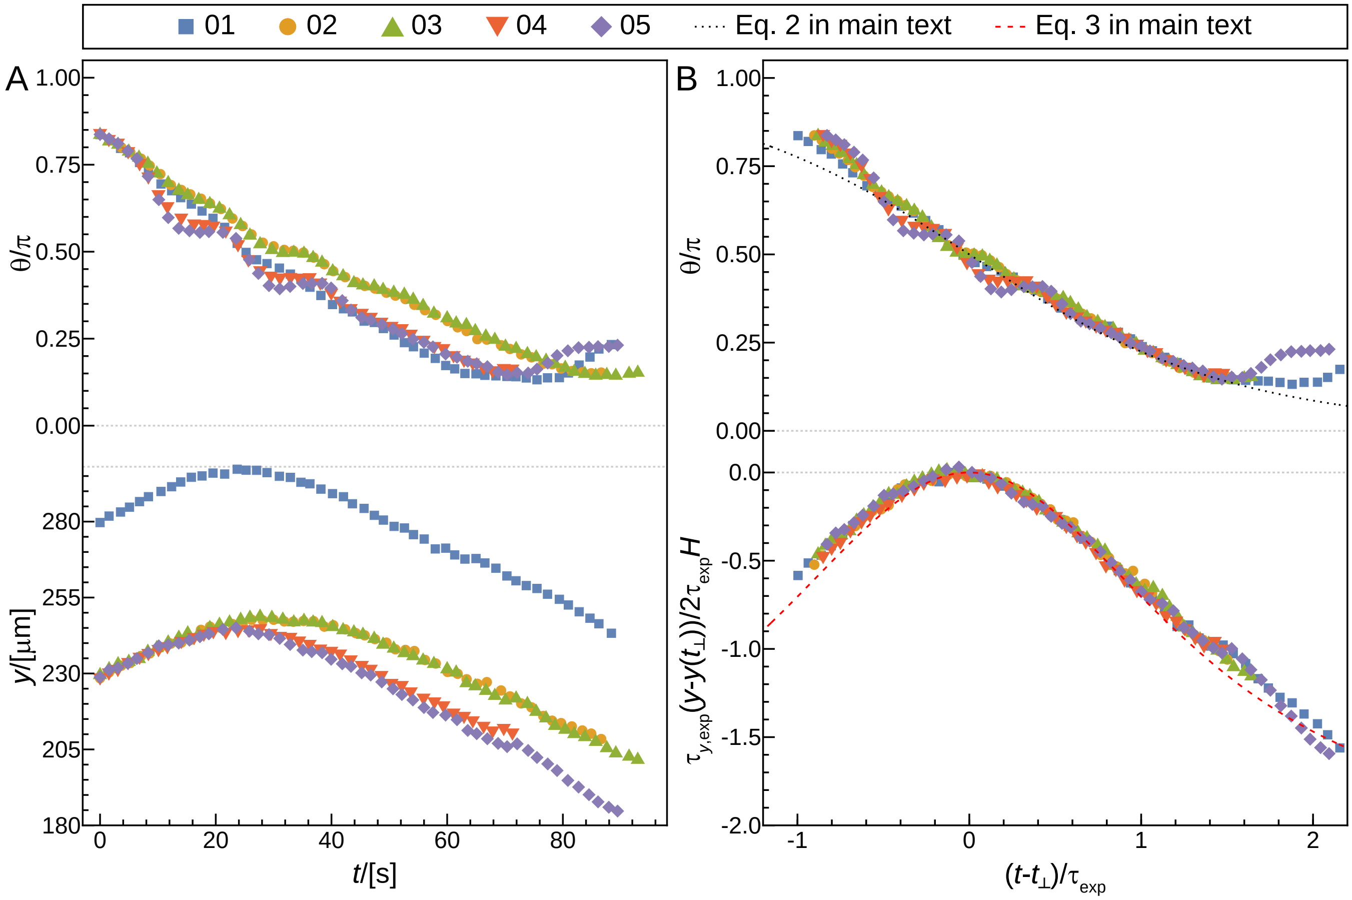


**Fig. S15. Raw and scaled experimental trajectories for a disk trimer with** $\kappa = 1.84$, $\phi = 51°$ (*A*) Orientation of the particle with respect to the flow (top) and its dimensional transversal position (bottom) as functions of real time. The transversal velocity of the particle changes sign at $\theta \approx \pi/2$. (*B*) Particle orientation (top) and scaled transversal position (bottom) as functions of scaled time. Both the rotation and translation of the particle are described well by equations 2 and 3 in the main text. Different experimental datasets are denoted by different numbers in the figure legend. In all cases the experimental uncertainty is smaller than the symbol size. The timescales used to re-scale each experimental dataset are given the Table S1.

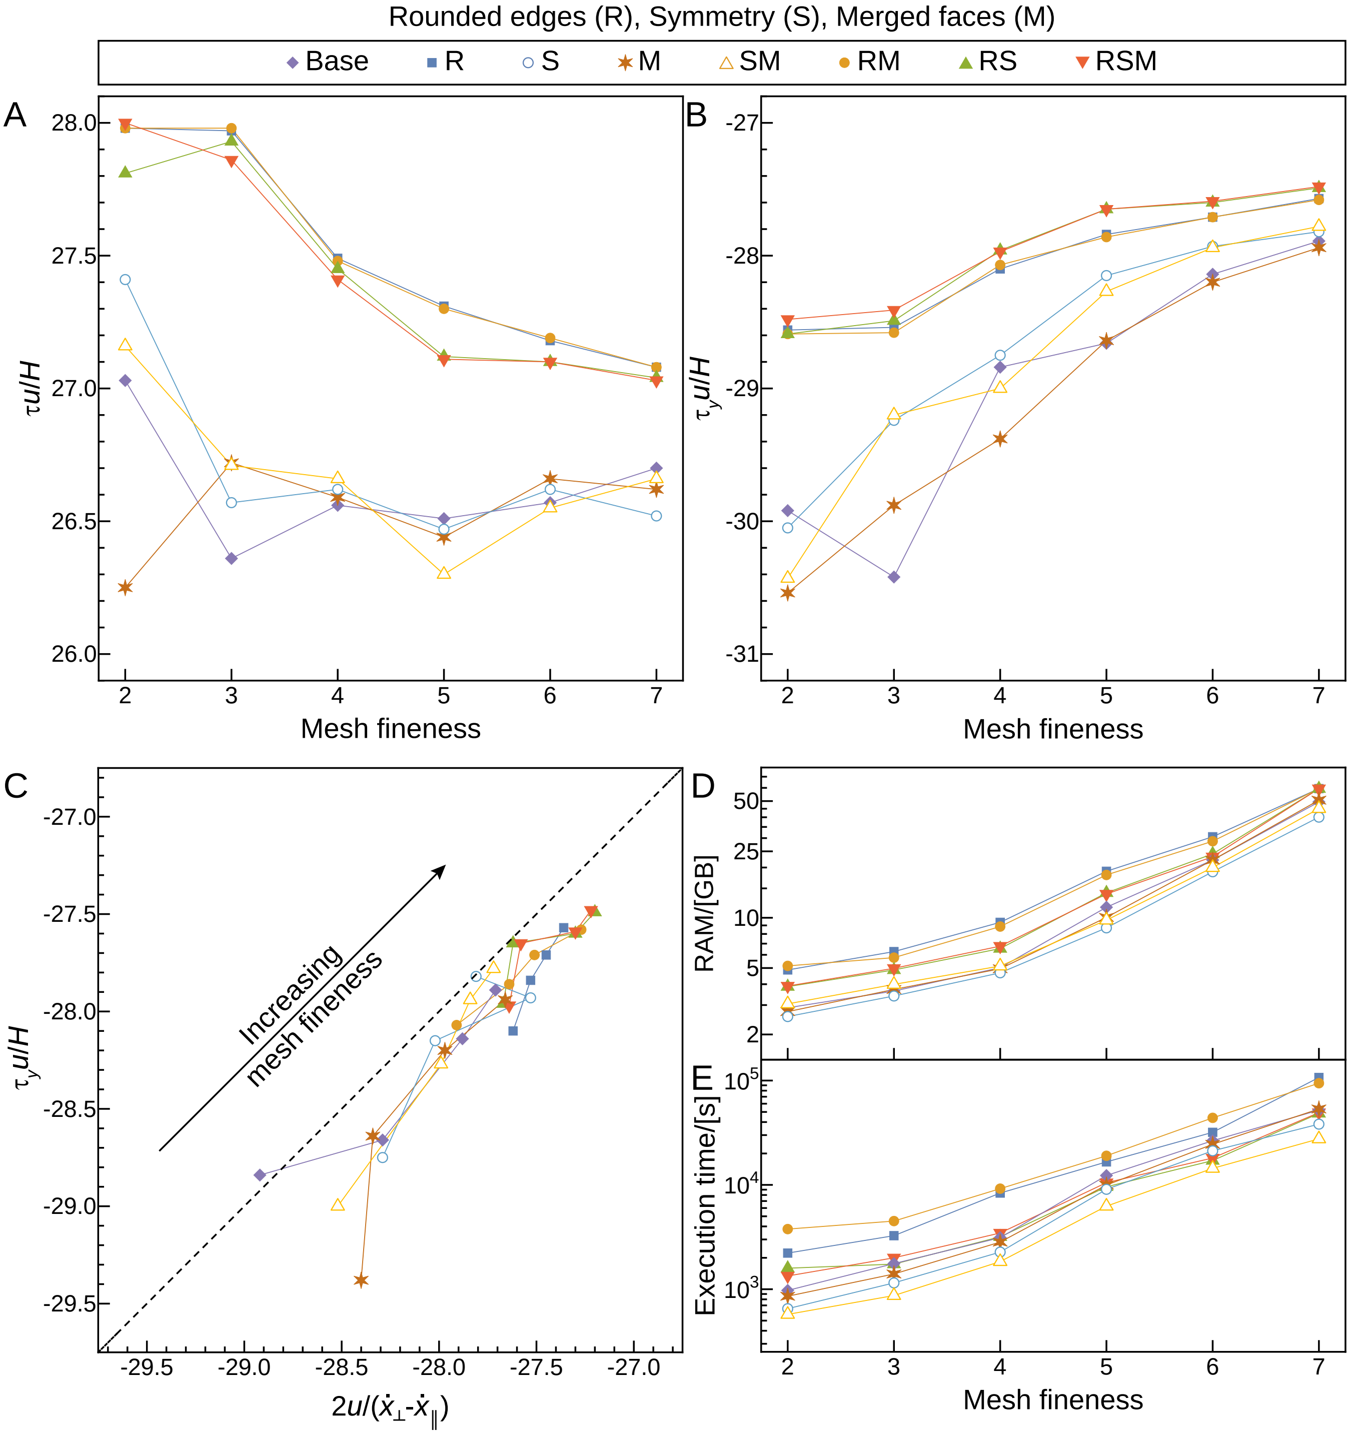


**Fig. S16. Convergence studies and performance of the finite element solver.** (*A*) The rotational $\tau$ and (*B*) translational timescales $\tau_y$ of a disk trimer are close to identical regardless of the optimization techniques applied to the particle geometry as long as a Fine mesh is used, corresponding to mesh fineness of 6. (*C*) We verify the assumption in SI Text 1D by comparing the dimensionless transversal timescale to the one computed via equation (16). Due to (*D*) memory and (*E*) execution time limitation, we choose to perform all computations using particles with rounded edges and merged faces, while exploiting symmetry along the channel height.

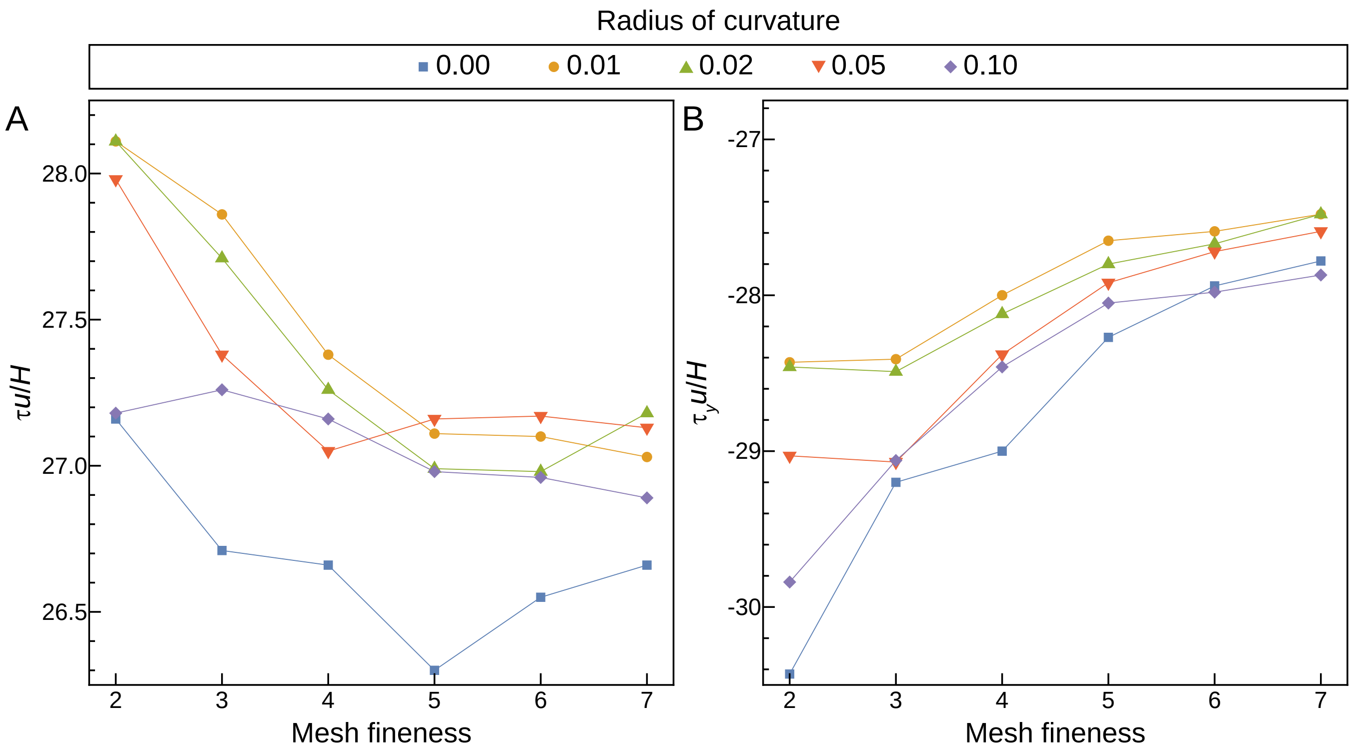


**Fig. S17. Effect of edge curvature on particle timescales.** Both (*A*) the rotational $\tau$ and (*B*) translational timescale $\tau_y$ depend weakly on edge curvature provided a sufficiently fine mesh is used.

 

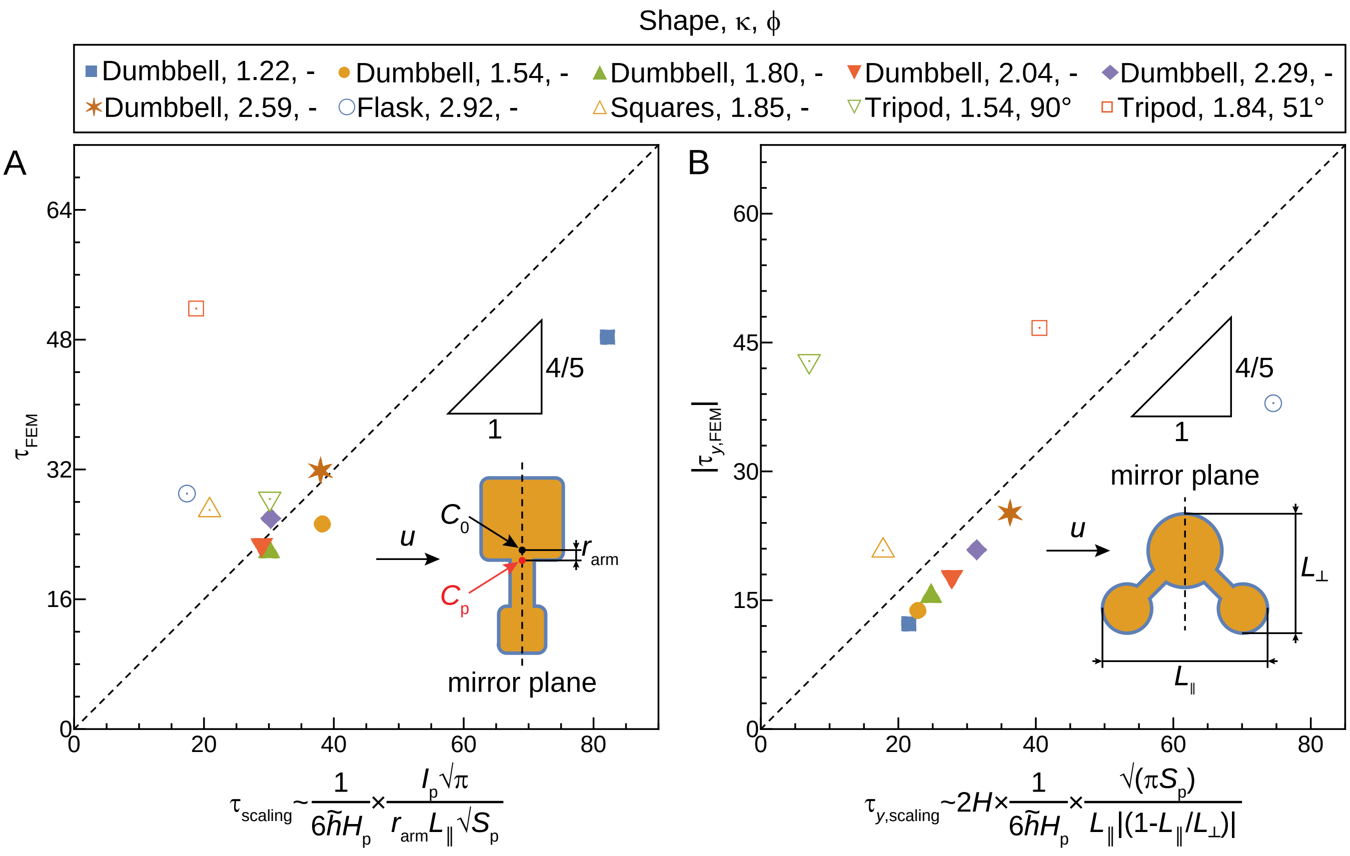


**Fig. S18. Comparison between timescales obtained with finite element calculations and minimalistic scaling relations.** For disk dimers the proposed relations overestimate both (*A*) the rotational $\tau$ and (*B*) translational $\tau_y$ timescales by roughly 20%. The mismatch between scalings and 3D FEM becomes more pronounced the more the particle deviates from a rod. The insets in both subfigures illustrate the geometric parameters used in the scalings.

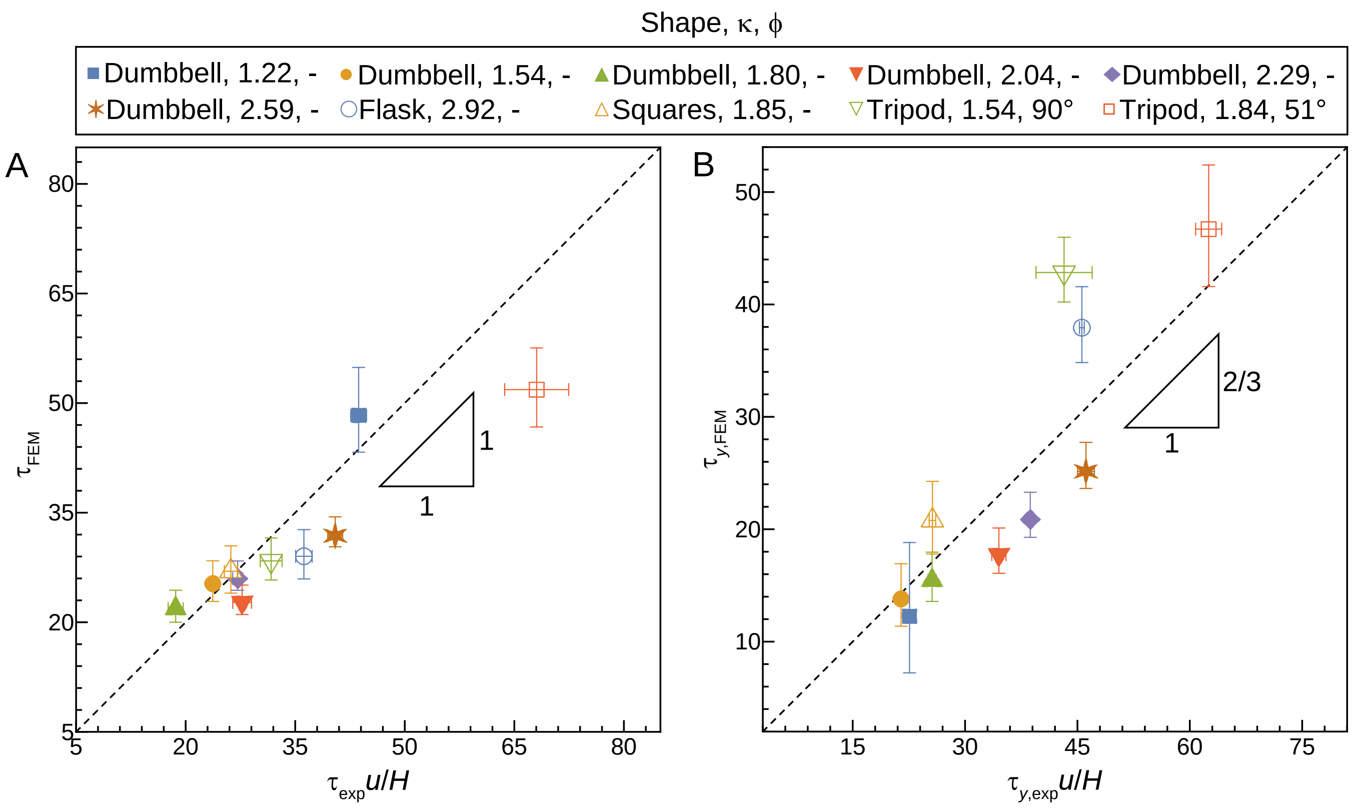


**Fig. S19. Comparison between timescales obtained from finite element calculations and from experiments.** While there is good agreement between computations and experiments for (*A*) the rotational timescales $\tau$, (*B*) the computed translational timescales $\tau_{y,\mathrm{FEM}}$ underestimate the experimental results by roughly 50% . The horizontal error bars represent the standard deviation of the timescales within an experimental series given in Table S1. The vertical error bars take into account the uncertainty in confinement of the particle: the upper value is the timescales computed for $h_{\mathrm{g}} + 0.5\,\mu\mathrm{m}$ and the lower value is the timescale computed for $h_{\mathrm{g}} - 0.5\,\mu\mathrm{m}$.

**Table S1. Rotational $\tau$ and translational $\tau_y$ timescales for various particle shapes.**

| Particle shape | Experiment | $u / \left[\mu m\, s^{-1}\right]$ | Frames | $\tau$ / [s] | $R^2$ ($\tau$) | $\tau_y$ / [s] | $R^2$ ($\tau_y$) |
|---|---|---|---|---|---|---|---|
| Disk dimer $\kappa = 1.22$ | 01 | 35 | 692 | 34.3±0.1 | 0.998 | 17.2±0.1 | 0.998 |
| | 02 | | 707 | 36.7±0.2 | 0.996 | 18.7±0.1 | 0.999 |
| | 03 | | 754 | 34.8±0.1 | 0.997 | 18.2±0.1 | 0.998 |
| | 04 | | 730 | 34.7±0.2 | 0.997 | 18.4±0.1 | 0.998 |
| Disk dimer $\kappa = 1.54$ | 01 | 55 | 388 | 13.0±0.1 | 0.990 | 12.0±0.0 | 0.998 |
| | 02 | | 403 | 12.8±0.1 | 0.994 | 11.3±0.0 | 0.998 |
| | 03 | | 413 | 12.4±0.1 | 0.989 | 11.7±0.0 | 0.999 |
| | 04 | | 395 | 12.6±0.1 | 0.993 | 11.0±0.0 | 0.998 |
| Disk dimer $\kappa = 1.80$ | 01 | 55 | 435 | 10.1±0.1 | 0.989 | 14.±0.1 | 0.997 |
| | 02 | | 660 | 12.0±0.1 | 0.994 | 12.8±0.1 | 0.996 |
| | 03 | | 349 | 9.3±0.1 | 0.991 | 13.3±0.1 | 0.996 |
| | 04 | | 373 | 9.6±0.1 | 0.990 | 13.9±0.1 | 0.995 |
| | 05 | | 351 | 9.3±0.1 | 0.988 | 14.2±0.1 | 0.991 |
| | 06 | | 366 | 9.6±0.1 | 0.990 | 14.0±0.1 | 0.994 |
| Disk dimer $\kappa = 2.04$ | 01 | 55 | 514 | 16.4±0.1 | 0.995 | 18.5±0.1 | 0.998 |
| | 02 | | 590 | 13.9±0.1 | 0.993 | 18.8±0.1 | 0.995 |
| | 03 | | 515 | 13.1±0.1 | 0.994 | 17.9±0.1 | 0.996 |
| | 04 | | 552 | 15.5±0.1 | 0.994 | 19.9±0.1 | 0.998 |
| | 05 | | 791 | 15.9±0.1 | 0.996 | 17.1±0.1 | 0.998 |
| | 06 | | 572 | 14.3±0.1 | 0.994 | 18.8±0.1 | 0.997 |
| Disk dimer $\kappa = 2.29$ | 01 | 55 | 428 | 14.5±0.1 | 0.991 | 20.9±0.2 | 0.990 |
| | 02 | | 479 | 14.5±0.1 | 0.992 | 20.4±0.1 | 0.994 |
| | 03 | | 425 | 15.4±0.1 | 0.992 | 20.3±0.2 | 0.994 |
| | 04 | | 563 | 14.7±0.1 | 0.991 | 21.1±0.2 | 0.990 |
| | 05 | | 534 | 13.5±0.1 | 0.991 | 21.0±0.2 | 0.990 |
| Disk dimer $\kappa = 2.59$ | 01 | 35 | 765 | 27.4±0.2 | 0.992 | 34.5±0.1 | 0.998 |
| | 02 | 70 | 605 | 14.9±0.1 | 0.996 | 17.9±0.1 | 0.995 |
| | 03 | | 558 | 15.3±0.1 | 0.997 | 16.4±0.4 | 0.908 |
| | 04 | | 488 | 14.6±0.1 | 0.997 | 15.9±0.1 | 0.998 |
| | 05 | | 579 | 15.5±0.1 | 0.991 | 16.8±0.1 | 0.988 |
| Triangular dimer $\kappa = 2.92$ | 01 | 55 | 1043 | 19.8±0.1 | 0.991 | 26.6±0.2 | 0.989 |
| | 02 | | 1119 | 21.2±0.1 | 0.988 | 26.6±0.1 | 0.995 |
| | 03 | | 1155 | 22.3±0.1 | 0.988 | 27.3±0.1 | 0.994 |
| | 04 | | 1171 | 21.9±0.1 | 0.988 | 26.9±0.1 | 0.995 |
| Square dimer $\kappa = 1.85$ | 01 | 70 | 380 | 11.1±0.0 | 1.000 | 11.7±0.1 | 0.997 |
| | 02 | | 541 | 12.4±0.2 | 0.978 | 11.8±0.2 | 0.953 |
| | 03 | | 342 | 12.9±0.0 | 1.000 | 12.2±0.1 | 0.997 |
| | 04 | | 341 | 13.0±0.0 | 1.000 | 12.6±0.1 | 0.995 |
| Disk trimer $\kappa = 1.54$ $\phi = 90°$ | 01 | 70 | 260 | 13.2±0.3 | 0.980 | -24.4±0.8 | 0.913 |
| | 02 | | 241 | 15.7±0.4 | 0.976 | -19.9±0.8 | 0.888 |
| | 03 | | 260 | 15.9±0.4 | 0.969 | -16.9±0.7 | 0.872 |
| | 04 | | 284 | 14.9±0.2 | 0.982 | -20.3±1.4 | 0.431 |
| | 05 | | 276 | 14.5±0.3 | 0.981 | -14.6±1.0 | 0.417 |
| Disk trimer $\kappa = 1.84$ $\phi = 51°$ | 01 | 70 | 1133 | 26.3±0.2 | 0.983 | 28.8±0.2 | 0.986 |
| | 02 | | 1489 | 36.0±0.3 | 0.974 | 31.9±0.1 | 0.992 |
| | 03 | | 1547 | 36.9±0.3 | 0.971 | 30.2±0.2 | 0.988 |
| | 04 | | 1209 | 30.6±0.4 | 0.957 | 29.2±0.2 | 0.988 |
| | 05 | | 1241 | 30.6±0.4 | 0.952 | 27.2±0.2 | 0.984 |

For each of the ten studied shapes, per experiment, we report the total number of processed frames, the timescales with their respective 95%-confidence intervals and the corresponding coefficients of determination. The average flow velocity $u$ is measured by tracking fluorescent microspheres.

## References


1. B Bet, S Samin, R Georgiev, HB Eral, R van Roij, Steering particles by breaking symmetries. *J. Phys. Condens. Matter* **30**, 224002 (2018).
2. H Brenner, The Stokes resistance of an arbitrary particle. *Chem. Eng. Sci.* **18**, 1–25 (1963).
3. WE Uspal, PS Doyle, Self-organizing microfluidic crystals. *Soft matter* **10**, 5177–5191 (2014).
4. B Bet, et al., Calculating the motion of highly confined, arbitrary-shaped particles in Hele–Shaw channels. *Microfluid. Nanofluid* **22**, 77 (2018).
5. WE Uspal, HB Eral, PS Doyle, Engineering particle trajectories in microfluidic flows using particle shape. *Nat. Commun.* **4**, 2666 (2013).
6. H Berthet, M Fermigier, A Lindner, Single fiber transport in a confined channel: Microfluidic experiments and numerical study. *Phys. Fluids* **25** (2013).
7. M Nagel, et al., Oscillations of confined fibres transported in microchannels. *J. Fluid Mech.* **835**, 444–470 (2018).
8. PR Amestoy, IS Duff, J Koster, JY L'Excellent, A fully asynchronous multifrontal solver using distributed dynamic scheduling. *SIAM J. Matrix Anal. Appl.* **23**, 15–41 (2001).
9. PR Amestoy, A Guermouche, JY L'Excellent, S Pralet, Hybrid scheduling for the parallel solution of linear systems. *Parallel Comput.* **32**, 136–156 (2006).
10. E Holzbecher, H Si, Accuracy Tests for COMSOL - and Delaunay Meshes in *Proceedings of the COMSOL Conference.* (Hanover), No. 1, p. 7 (2008).
11. T Beatus, RH Bar-Ziv, T Tlusty, The physics of 2D microfluidic droplet ensembles. *Phys. Rep.* **516**, 103–145 (2012).
